# Supplementary material for: Learning to Project for Cross-Task Knowledge Distillation
Source: arXiv:2403.14494 source file (2024-11-27)
Supplement: Supplementary file 1 [file main.tex]

\clearpage

%%%%%%%% CHANGE THESE TWO COMMANDS FOR CAMERA READY
\setcounter{page}{1}
\section{Supplementary Material: Learning to Project for Cross-Task Knowledge Distillation (Submission 448)}

\subsection{Code}
\label{sec:app:code}
    We include our anonymised code in the accompanying .zip file, and will release it publicly upon acceptance. Our codebase is written in Python using PyTorch \cite{paszke_pytorch_2019} and is based on several other codebases:
    \begin{itemize}
        \item \textbf{Monocular depth estimation student:} we build on the codebase of AiT \cite{ning_all_2023}, which is built in turn on MMDetection \cite{mmdetection_contributors_openmmlab_2018}. No license is specified in the original AiT repository. MMDetection is released under the Apache license.
        \item \textbf{Semantic segmentation:} our code builds on the pipeline of \\ \url{github.com/yassouali/pytorch-segmentation} \\(released under MIT license).
        \item \textbf{Image-to-image translation:} our code builds on the official PyTorch implementation of Pix2Pix and CycleGAN (released under the BSD license):\\ \url{github.com/junyanz/pytorch-CycleGAN-and-pix2pix}
    \end{itemize}

    A full README is included in the code release, and includes instructions for setup, evaluation, and training.

\subsection{Full monocular depth estimation results}
\label{sec:app:full-results}
    
    Table \ref{tab:main_cross_task_distillation} shows only some metrics for monocular depth estimation (MDE) on NYUv2 \cite{silberman_indoor_2012} for the sake of brevity. We include here four additional tables showing the performance on all available metrics of a depth estimation student when distilled to from teachers trained for different tasks. Each table also includes metrics for the baseline, which is a student model trained without any distillation setup of any kind (i.e. only the task loss $\mathcal{L}_{task}$ is used). 
    Full details of the metrics used are in section \ref{sec:app:metrics}.
    See section \ref{sec:app:depth-student-models} for complete architectural details and section \ref{sec:app:loss-functions} for loss function details.

    \begin{table}
    \centering
    \scriptsize
    \begin{tabular}{ll|lllllll}
        \toprule
        \belowrulesepcolor{mygrey}
        \rowcolor{mygrey}
         &
           &
          \multicolumn{7}{c}{{\color{d2d} $\blacksquare$ } \textbf{Depth \textit{(Most similar)}} $\longrightarrow$ Depth} \\
        \rowcolor{mygrey} Method &
        Projection type &
          $\delta_1 \uparrow$ &
          $\delta_2 \uparrow$ &
          \multicolumn{1}{l|}{$\delta_3 \uparrow$} &
          Abs. Rel. $\downarrow$ &
          Sq. Rel. $\downarrow$ &
          RMS $\downarrow$ &
          RMSL $\downarrow$ \\ 
        \aboverulesepcolor{mygrey}
        \midrule
        \multicolumn{2}{c|}{\textit{No teacher (baseline)}} &
          \stackengine{2pt}{\textit{0.845}}{$_{\pm 0.007}$}{U}{c}{F}{T}{S} &
          \stackengine{2pt}{\textit{0.974}}{$_{\pm 0.001}$}{U}{c}{F}{T}{S} &
          \multicolumn{1}{l|}{\stackengine{2pt}{\textit{0.995}}{$_{\pm 0.000}$}{U}{c}{F}{T}{S}} &
          \stackengine{2pt}{\textit{0.127}}{$_{\pm 0.003}$}{U}{c}{F}{T}{S} &
          \stackengine{2pt}{\textit{0.078}}{$_{\pm 0.002}$}{U}{c}{F}{T}{S} &
          \stackengine{2pt}{\textit{0.440}}{$_{\pm 0.005}$}{U}{c}{F}{T}{S} &
          \stackengine{2pt}{\textit{0.160}}{$_{\pm 0.003}$}{U}{c}{F}{T}{S} \\
        \midrule
         &
          Traditional &
          \textbf{0.868} &
          \textbf{0.979} &
          \multicolumn{1}{l|}{\textbf{0.996}} &
          \textbf{0.117} &
          \textbf{0.069} &
          \textbf{0.406} &
          \textbf{0.148} \\
         &
          Inverted (Ours) &
          0.849 &
          0.976 &
          \multicolumn{1}{l|}{0.995} &
          0.124 &
          0.075 &
          0.432 &
          0.157 \\
        \multirow{-3}{*}{\begin{tabular}[c]{@{}l@{}}FitNets~\cite{romero_fitnets_2015} \\     \textit{\scriptsize ICLR 2015}\end{tabular}} &
          \textit{Improvement} &
          \cellcolor[HTML]{FFB0B0}\textit{-2.17\%} &
          \cellcolor[HTML]{FFF2F2}\textit{-0.34\%} &
          \multicolumn{1}{l|}{\cellcolor[HTML]{FFFEFE}\textit{-0.01\%}} &
          \cellcolor[HTML]{FF5858}\textit{-6.35\%} &
          \cellcolor[HTML]{FF5858}\textit{-9.66\%} &
          \cellcolor[HTML]{FF5858}\textit{-6.49\%} &
          \cellcolor[HTML]{FF5858}\textit{-5.92\%} \\ \midrule
         &
          Traditional &
          \textbf{0.856} &
          0.976 &
          \multicolumn{1}{l|}{\textbf{0.995}} &
          \textbf{0.122} &
          \textbf{0.073} &
          0.426 &
          \textbf{0.155} \\
         &
          Inverted (Ours) &
          \textbf{0.856} &
          \textbf{0.977} &
          \multicolumn{1}{l|}{\textbf{0.995}} &
          \textbf{0.122} &
          \textbf{0.073} &
          \textbf{0.425} &
          \textbf{0.155} \\
        \multirow{-3}{*}{\begin{tabular}[c]{@{}l@{}}AT~\cite{Zagoruyko2019PayingTransfer} \\  \textit{\scriptsize ICLR 2017}\end{tabular}} &
          \textit{Improvement} &
          \cellcolor[HTML]{FFFBFB}\textit{-0.11\%} &
          \cellcolor[HTML]{FDFFFD}\textit{0.06\%} &
          \multicolumn{1}{l|}{\cellcolor[HTML]{FFFFFF}\textit{0.01\%}} &
          \cellcolor[HTML]{FFFCFC}\textit{-0.08\%} &
          \cellcolor[HTML]{E2FFE2}\textit{0.82\%} &
          \cellcolor[HTML]{FFFFFF}\textit{0.02\%} &
          \cellcolor[HTML]{FFFFFF}\textit{0.00\%} \\ \midrule
         &
          Traditional &
          \textbf{0.854} &
          \textbf{0.978} &
          \multicolumn{1}{l|}{\textbf{0.996}} &
          \textbf{0.122} &
          \textbf{0.072} &
          0.429 &
          \textbf{0.155} \\
         &
          Inverted (Ours) &
          \textbf{0.854} &
          0.977 &
          \multicolumn{1}{l|}{\textbf{0.996}} &
          \textbf{0.122} &
          0.073 &
          \textbf{0.427} &
          \textbf{0.155} \\
        \multirow{-3}{*}{\begin{tabular}[c]{@{}l@{}}PKT~\cite{Passalis2018LearningTransfer} \\     \textit{\scriptsize ECCV 2018}\end{tabular}} &
          \textit{Improvement} &
          \cellcolor[HTML]{FEFFFE}\textit{0.04\%} &
          \cellcolor[HTML]{FFFBFB}\textit{-0.09\%} &
          \multicolumn{1}{l|}{\cellcolor[HTML]{FFFFFF}\textit{0.02\%}} &
          \cellcolor[HTML]{FFF9F9}\textit{-0.16\%} &
          \cellcolor[HTML]{FFCCCC}\textit{-1.38\%} &
          \cellcolor[HTML]{F0FFF0}\textit{0.42\%} &
          \cellcolor[HTML]{F8FFF8}\textit{0.19\%} \\ \midrule
         &
          Traditional &
          \textbf{0.861} &
          \textbf{0.978} &
          \multicolumn{1}{l|}{\textbf{0.996}} &
          \textbf{0.119} &
          \textbf{0.070} &
          \textbf{0.416} &
          \textbf{0.151} \\
         &
          Inverted (Ours) &
          0.849 &
          0.975 &
          \multicolumn{1}{l|}{\textbf{0.996}} &
          0.124 &
          0.076 &
          0.433 &
          0.157 \\
        \multirow{-3}{*}{\begin{tabular}[c]{@{}l@{}}Ensemble~\cite{Chen2022ImprovedEnsemble} \\    \textit{\scriptsize NeurIPS 2022}\end{tabular}} &
          \textit{Improvement} &
          \cellcolor[HTML]{FFC9C9}\textit{-1.46\%} &
          \cellcolor[HTML]{FFF4F4}\textit{-0.29\%} &
          \multicolumn{1}{l|}{\cellcolor[HTML]{FFFDFD}\textit{-0.05\%}} &
          \cellcolor[HTML]{FF5656}\textit{-4.64\%} &
          \cellcolor[HTML]{FF5858}\textit{-7.86\%} &
          \cellcolor[HTML]{FF6969}\textit{-4.11\%} &
          \cellcolor[HTML]{FF6464}\textit{-4.25\%} \\ 
          \bottomrule
    \end{tabular}
    \vspace{1em}
    \caption{\textbf{Depth teacher $\rightarrow$ Depth student (no task gap).} As expected, in same-task settings, our inverted projection produces a smaller improvement than the traditional projection. \textit{Improvement} is \% change using our inverted projection over using the traditional projection. See section \ref{sec:app:model_details} for model details. Baseline $\pm$ figures are variance from 3 runs.}
    \label{tab:supp:full-depth-table:depth-teacher}
\end{table}
\begin{table}
    \centering
    \scriptsize
    \begin{tabular}{ll|lllllll}
        \toprule
        \belowrulesepcolor{mygrey}
        \rowcolor{mygrey}
         &
           &
          \multicolumn{7}{c}{{\color{s2d} $\blacksquare$ } \textbf{Instance Segmentation} $\longrightarrow$ Depth} \\
        \rowcolor{mygrey} Method &
          Projection type &
          $\delta_1 \uparrow$ &
          $\delta_2 \uparrow$ &
          \multicolumn{1}{l|}{$\delta_3 \uparrow$} &
          Abs. Rel. $\downarrow$ &
          Sq. Rel. $\downarrow$ &
          RMS $\downarrow$ &
          RMSL $\downarrow$ \\  
        \aboverulesepcolor{mygrey}
        \midrule
        \multicolumn{2}{c|}{\textit{No teacher (baseline)}} &
          \stackengine{2pt}{\textit{0.845}}{$_{\pm 0.007}$}{U}{c}{F}{T}{S} &
          \stackengine{2pt}{\textit{0.974}}{$_{\pm 0.001}$}{U}{c}{F}{T}{S} &
          \multicolumn{1}{l|}{\stackengine{2pt}{\textit{0.995}}{$_{\pm 0.000}$}{U}{c}{F}{T}{S}} &
          \stackengine{2pt}{\textit{0.127}}{$_{\pm 0.003}$}{U}{c}{F}{T}{S} &
          \stackengine{2pt}{\textit{0.078}}{$_{\pm 0.002}$}{U}{c}{F}{T}{S} &
          \stackengine{2pt}{\textit{0.440}}{$_{\pm 0.005}$}{U}{c}{F}{T}{S} &
          \stackengine{2pt}{\textit{0.160}}{$_{\pm 0.003}$}{U}{c}{F}{T}{S} \\
         \midrule
         &
          Traditional &
          \textbf{0.855} &
          \textbf{0.977} &
          \multicolumn{1}{l|}{\textbf{0.996}} &
          \textbf{0.122} &
          \textbf{0.073} &
          \textbf{0.425} &
          \textbf{0.154} \\
         &
          Inverted (Ours) &
          0.851 &
          0.975 &
          \multicolumn{1}{l|}{0.995} &
          0.124 &
          0.075 &
          0.431 &
          0.157 \\
        \multirow{-3}{*}{\begin{tabular}[c]{@{}l@{}}FitNets~\cite{romero_fitnets_2015} \\     \textit{\scriptsize ICLR 2015}\end{tabular}} &
          \textit{Improvement} &
          \cellcolor[HTML]{FFF0F0}\textit{-0.41\%} &
          \cellcolor[HTML]{FFF5F5}\textit{-0.25\%} &
          \multicolumn{1}{l|}{\cellcolor[HTML]{FFFEFE}\textit{-0.02\%}} &
          \cellcolor[HTML]{FFBEBE}\textit{-1.78\%} &
          \cellcolor[HTML]{FFA3A3}\textit{-2.52\%} &
          \cellcolor[HTML]{FFCFCF}\textit{-1.31\%} &
          \cellcolor[HTML]{FFC1C1}\textit{-1.68\%} \\ \midrule
         &
          Traditional &
          0.852 &
          0.976 &
          \multicolumn{1}{l|}{\textbf{0.995}} &
          0.123 &
          0.075 &
          0.431 &
          0.156 \\
         &
          Inverted (Ours) &
          \textbf{0.855} &
          \textbf{0.978} &
          \multicolumn{1}{l|}{\textbf{0.995}} &
          \textbf{0.121} &
          \textbf{0.073} &
          \textbf{0.429} &
          \textbf{0.155} \\
        \multirow{-3}{*}{\begin{tabular}[c]{@{}l@{}}AT~\cite{Zagoruyko2019PayingTransfer} \\  \textit{\scriptsize ICLR 2017}\end{tabular}} &
          \textit{Improvement} &
          \cellcolor[HTML]{F0FFF0}\textit{0.42\%} &
          \cellcolor[HTML]{FAFFFA}\textit{0.16\%} &
          \multicolumn{1}{l|}{\cellcolor[HTML]{FFFFFF}\textit{0.00\%}} &
          \cellcolor[HTML]{CDFFCD}\textit{1.38\%} &
          \cellcolor[HTML]{C0FFC0}\textit{1.74\%} &
          \cellcolor[HTML]{ECFFEC}\textit{0.53\%} &
          \cellcolor[HTML]{E3FFE3}\textit{0.77\%} \\ \midrule
         &
          Traditional &
          \textbf{0.857} &
          \textbf{0.976} &
          \multicolumn{1}{l|}{\textbf{0.995}} &
          \textbf{0.123} &
          \textbf{0.075} &
          \textbf{0.427} &
          \textbf{0.155} \\
         &
          Inverted (Ours) &
          0.854 &
          \textbf{0.976} &
          \multicolumn{1}{l|}{\textbf{0.995}} &
          \textbf{0.123} &
          \textbf{0.075} &
          0.429 &
          0.156 \\
        \multirow{-3}{*}{\begin{tabular}[c]{@{}l@{}}PKT~\cite{Passalis2018LearningTransfer} \\     \textit{\scriptsize ECCV 2018}\end{tabular}} &
          \textit{Improvement} &
          \cellcolor[HTML]{FFF2F2}\textit{-0.34\%} &
          \cellcolor[HTML]{FEFFFE}\textit{0.04\%} &
          \multicolumn{1}{l|}{\cellcolor[HTML]{FFFFFF}\textit{0.01\%}} &
          \cellcolor[HTML]{FFFCFC}\textit{-0.08\%} &
          \cellcolor[HTML]{FFFAFA}\textit{-0.13\%} &
          \cellcolor[HTML]{FFEEEE}\textit{-0.44\%} &
          \cellcolor[HTML]{FFECEC}\textit{-0.52\%} \\ \midrule
         &
          Traditional &
          \textbf{0.856} &
          \textbf{0.977} &
          \multicolumn{1}{l|}{\textbf{0.996}} &
          \textbf{0.122} &
          \textbf{0.072} &
          \textbf{0.425} &
          \textbf{0.154} \\
         &
          Inverted (Ours) &
          0.848 &
          0.975 &
          \multicolumn{1}{l|}{0.995} &
          0.124 &
          0.076 &
          0.435 &
          0.157 \\
        \multirow{-3}{*}{\begin{tabular}[c]{@{}l@{}}Ensemble~\cite{Chen2022ImprovedEnsemble} \\     \textit{\scriptsize NeurIPS 2022}\end{tabular}} &
          \textit{Improvement} &
          \cellcolor[HTML]{FFDCDC}\textit{-0.95\%} &
          \cellcolor[HTML]{FFF9F9}\textit{-0.16\%} &
          \multicolumn{1}{l|}{\cellcolor[HTML]{FFFDFD}\textit{-0.05\%}} &
          \cellcolor[HTML]{FFC3C3}\textit{-1.64\%} &
          \cellcolor[HTML]{FF5353}\textit{-4.70\%} &
          \cellcolor[HTML]{FFB0B0}\textit{-2.16\%} &
          \cellcolor[HTML]{FFBABA}\textit{-1.88\%} \\
          \bottomrule
    \end{tabular}
    \vspace{1em}
    \caption{\textbf{Instance segmentation teacher $\rightarrow$ Depth student (small task gap).} The two tasks are different, but are similar enough that the traditional projection produces greater improvements than our inverted projection does with most methods. \textit{Improvement} is \% change using our inverted projection over using the traditional projection. See section \ref{sec:app:model_details} for model details. Baseline $\pm$ figures are variance from 3 runs.}
    \label{tab:supp:full-depth-table:insseg-teacher}
\end{table}
\begin{table}
    \centering
    \scriptsize
    \begin{tabular}{ll|lllllll}
        \toprule
        \belowrulesepcolor{mygrey}
        \rowcolor{mygrey}
         &
           &
          \multicolumn{7}{c}{{\color{c2d} $\blacksquare$ } \textbf{Classification} $\longrightarrow$ Depth} \\
        \rowcolor{mygrey} Method &
          Projection type &
          $\delta_1 \uparrow$ &
          $\delta_2 \uparrow$ &
          \multicolumn{1}{l|}{$\delta_3 \uparrow$} &
          Abs. Rel. $\downarrow$ &
          Sq. Rel. $\downarrow$ &
          RMS $\downarrow$ &
          RMSL $\downarrow$ \\ 
        \aboverulesepcolor{mygrey}
        \midrule
        \multicolumn{2}{c|}{\textit{No teacher (baseline)}} &
          \stackengine{2pt}{\textit{0.845}}{$_{\pm 0.007}$}{U}{c}{F}{T}{S} &
          \stackengine{2pt}{\textit{0.974}}{$_{\pm 0.001}$}{U}{c}{F}{T}{S} &
          \multicolumn{1}{l|}{\stackengine{2pt}{\textit{0.995}}{$_{\pm 0.000}$}{U}{c}{F}{T}{S}} &
          \stackengine{2pt}{\textit{0.127}}{$_{\pm 0.003}$}{U}{c}{F}{T}{S} &
          \stackengine{2pt}{\textit{0.078}}{$_{\pm 0.002}$}{U}{c}{F}{T}{S} &
          \stackengine{2pt}{\textit{0.440}}{$_{\pm 0.005}$}{U}{c}{F}{T}{S} &
          \stackengine{2pt}{\textit{0.160}}{$_{\pm 0.003}$}{U}{c}{F}{T}{S} \\
         \midrule
         &
          Traditional &
          0.845 &
          \textbf{0.976} &
          \multicolumn{1}{l|}{\textbf{0.996}} &
          0.125 &
          0.076 &
          0.439 &
          0.158 \\
         &
          Inverted (Ours) &
          \textbf{0.850} &
          0.975 &
          \multicolumn{1}{l|}{\textbf{0.995}} &
          \textbf{0.124} &
          \textbf{0.075} &
          \textbf{0.434} &
          \textbf{0.157} \\
        \multirow{-3}{*}{\begin{tabular}[c]{@{}l@{}}FitNets~\cite{romero_fitnets_2015} \\     \textit{\scriptsize ICLR 2015}\end{tabular}} &
          \textit{Improvement} &
          \cellcolor[HTML]{EDFFED}\textit{0.50\%} &
          \cellcolor[HTML]{FFFCFC}\textit{-0.06\%} &
          \multicolumn{1}{l|}{\cellcolor[HTML]{FFFDFD}\textit{-0.03\%}} &
          \cellcolor[HTML]{ECFFEC}\textit{0.53\%} &
          \cellcolor[HTML]{EFFFEF}\textit{0.44\%} &
          \cellcolor[HTML]{CFFFCF}\textit{1.34\%} &
          \cellcolor[HTML]{E2FFE2}\textit{0.80\%} \\ \midrule
         &
          Traditional &
          0.850 &
          \textbf{0.976} &
          \multicolumn{1}{l|}{\textbf{0.995}} &
          0.125 &
          0.076 &
          0.433 &
          0.157 \\
         &
          Inverted (Ours) &
          \textbf{0.853} &
          \textbf{0.976} &
          \multicolumn{1}{l|}{\textbf{0.995}} &
          \textbf{0.123} &
          \textbf{0.074} &
          \textbf{0.430} &
          \textbf{0.156} \\
        \multirow{-3}{*}{\begin{tabular}[c]{@{}l@{}}AT~\cite{Zagoruyko2019PayingTransfer} \\ \textit{\scriptsize ICLR 2017}\end{tabular}} &
          \textit{Improvement} &
          \cellcolor[HTML]{F3FFF3}\textit{0.35\%} &
          \cellcolor[HTML]{FDFFFD}\textit{0.08\%} &
          \multicolumn{1}{l|}{\cellcolor[HTML]{FFFFFF}\textit{0.02\%}} &
          \cellcolor[HTML]{C5FFC5}\textit{1.61\%} &
          \cellcolor[HTML]{91FF91}\textit{3.03\%} &
          \cellcolor[HTML]{E3FFE3}\textit{0.79\%} &
          \cellcolor[HTML]{E1FFE1}\textit{0.83\%} \\ \midrule
         &
          Traditional &
          0.851 &
          0.975 &
          \multicolumn{1}{l|}{\textbf{0.996}} &
          0.124 &
          0.076 &
          0.432 &
          0.157 \\
         &
          Inverted (Ours) &
          \textbf{0.853} &
          \textbf{0.976} &
          \multicolumn{1}{l|}{0.995} &
          \textbf{0.123} &
          \textbf{0.074} &
          \textbf{0.431} &
          \textbf{0.156} \\
        \multirow{-3}{*}{\begin{tabular}[c]{@{}l@{}}PKT~\cite{Passalis2018LearningTransfer} \\     \textit{\scriptsize ECCV 2018}\end{tabular}} &
          \textit{Improvement} &
          \cellcolor[HTML]{F7FFF7}\textit{0.25\%} &
          \cellcolor[HTML]{FEFFFE}\textit{0.05\%} &
          \multicolumn{1}{l|}{\cellcolor[HTML]{FFFDFD}\textit{-0.03\%}} &
          \cellcolor[HTML]{D1FFD1}\textit{1.29\%} &
          \cellcolor[HTML]{A5FFA5}\textit{2.50\%} &
          \cellcolor[HTML]{F5FFF5}\textit{0.30\%} &
          \cellcolor[HTML]{E8FFE8}\textit{0.64\%} \\ \midrule
         &
          Traditional &
          \textbf{0.852} &
          \textbf{0.976} &
          \multicolumn{1}{l|}{\textbf{0.995}} &
          \textbf{0.124} &
          \textbf{0.075} &
          \textbf{0.431} &
          \textbf{0.156} \\
         &
          Inverted (Ours) &
          0.847 &
          0.975 &
          \multicolumn{1}{l|}{\textbf{0.995}} &
          0.125 &
          0.076 &
          0.437 &
          0.158 \\
        \multirow{-3}{*}{\begin{tabular}[c]{@{}l@{}}Ensemble~\cite{Chen2022ImprovedEnsemble} \\     \textit{\scriptsize NeurIPS 2022}\end{tabular}} &
          \textit{Improvement} &
          \cellcolor[HTML]{FFE7E7}\textit{-0.63\%} &
          \cellcolor[HTML]{FFFAFA}\textit{-0.12\%} &
          \multicolumn{1}{l|}{\cellcolor[HTML]{FFFFFF}\textit{0.02\%}} &
          \cellcolor[HTML]{FFDEDE}\textit{-0.89\%} &
          \cellcolor[HTML]{FFC4C4}\textit{-1.61\%} &
          \cellcolor[HTML]{FFCFCF}\textit{-1.30\%} &
          \cellcolor[HTML]{FFD7D7}\textit{-1.09\%} \\
          \bottomrule
    \end{tabular}
    \vspace{1em}
    \caption{\textbf{Classification teacher $\rightarrow$ Depth student (larger task gap).} The two tasks are different enough that the setting becomes more ``cross-task" than ``same-task", and our inverted projection begins to outperform the traditional student model in terms of improvement over the baseline. \textit{Improvement} is \% change using our inverted projection over using the traditional projection. See section \ref{sec:app:model_details} for model details. Baseline $\pm$ figures are variance from 3 runs.}
    \label{tab:supp:full-depth-table:class-teacher}
\end{table}
\begin{table}
    \centering
    \scriptsize
    \begin{tabular}{ll|lllllll}
        \toprule
        \belowrulesepcolor{mygrey}
        \rowcolor{mygrey}
         &
           &
          \multicolumn{7}{c}{{\color{r2d} $\blacksquare$ } \textbf{Random \textit{(Least similar)}} $\longrightarrow$ Depth} \\
        \rowcolor{mygrey} Method &
          Projection type &
          $\delta_1 \uparrow$ &
          $\delta_2 \uparrow$ &
          \multicolumn{1}{l|}{$\delta_3 \uparrow$} &
          Abs. Rel. $\downarrow$ &
          Sq. Rel. $\downarrow$ &
          RMS $\downarrow$ &
          RMSL $\downarrow$ \\ 
        \aboverulesepcolor{mygrey}
        \midrule
        \multicolumn{2}{c|}{\textit{No teacher (baseline)}} &
          \stackengine{2pt}{\textit{0.845}}{$_{\pm 0.007}$}{U}{c}{F}{T}{S} &
          \stackengine{2pt}{\textit{0.974}}{$_{\pm 0.001}$}{U}{c}{F}{T}{S} &
          \multicolumn{1}{l|}{\stackengine{2pt}{\textit{0.995}}{$_{\pm 0.000}$}{U}{c}{F}{T}{S}} &
          \stackengine{2pt}{\textit{0.127}}{$_{\pm 0.003}$}{U}{c}{F}{T}{S} &
          \stackengine{2pt}{\textit{0.078}}{$_{\pm 0.002}$}{U}{c}{F}{T}{S} &
          \stackengine{2pt}{\textit{0.440}}{$_{\pm 0.005}$}{U}{c}{F}{T}{S} &
          \stackengine{2pt}{\textit{0.160}}{$_{\pm 0.003}$}{U}{c}{F}{T}{S} \\
         \midrule
         &
          Traditional &
          0.828 &
          0.970 &
          \multicolumn{1}{l|}{\textbf{0.995}} &
          0.134 &
          0.084 &
          0.455 &
          0.167 \\
         &
          Inverted (Ours) &
          \textbf{0.851} &
          \textbf{0.976} &
          \multicolumn{1}{l|}{\textbf{0.995}} &
          \textbf{0.124} &
          \textbf{0.075} &
          \textbf{0.431} &
          \textbf{0.156} \\
        \multirow{-3}{*}{\begin{tabular}[c]{@{}l@{}}FitNets~\cite{romero_fitnets_2015} \\     \textit{\scriptsize ICLR 2015}\end{tabular}} &
          \textit{Improvement} &
          \cellcolor[HTML]{97FF97}\textit{2.86\%} &
          \cellcolor[HTML]{EAFFEA}\textit{0.58\%} &
          \multicolumn{1}{l|}{\cellcolor[HTML]{FDFFFD}\textit{0.08\%}} &
          \cellcolor[HTML]{00FF00}\textit{7.47\%} &
          \cellcolor[HTML]{00FF00}\textit{11.15\%} &
          \cellcolor[HTML]{42FF42}\textit{5.20\%} &
          \cellcolor[HTML]{18FF18}\textit{6.36\%} \\ \midrule
         &
          Traditional &
          \textbf{0.857} &
          \textbf{0.977} &
          \multicolumn{1}{l|}{\textbf{0.996}} &
          \textbf{0.121} &
          \textbf{0.073} &
          \textbf{0.428} &
          \textbf{0.154} \\
         &
          Inverted (Ours) &
          \textbf{0.857} &
          0.976 &
          \multicolumn{1}{l|}{0.995} &
          0.122 &
          0.074 &
          \textbf{0.428} &
          0.155 \\
        \multirow{-3}{*}{\begin{tabular}[c]{@{}l@{}}AT~\cite{Zagoruyko2019PayingTransfer} \\ \textit{\scriptsize ICLR 2017}\end{tabular}} &
          \textit{Improvement} &
          \cellcolor[HTML]{FEFFFE}\textit{0.05\%} &
          \cellcolor[HTML]{FFFDFD}\textit{-0.04\%} &
          \multicolumn{1}{l|}{\cellcolor[HTML]{FFFDFD}\textit{-0.03\%}} &
          \cellcolor[HTML]{FFE0E0}\textit{-0.83\%} &
          \cellcolor[HTML]{FFCCCC}\textit{-1.37\%} &
          \cellcolor[HTML]{FCFFFC}\textit{0.09\%} &
          \cellcolor[HTML]{FFF0F0}\textit{-0.39\%} \\ \midrule
         &
          Traditional &
          0.856 &
          0.975 &
          \multicolumn{1}{l|}{\textbf{0.995}} &
          0.123 &
          0.075 &
          0.429 &
          \textbf{0.155} \\
         &
          Inverted (Ours) &
          \textbf{0.858} &
          \textbf{0.976} &
          \multicolumn{1}{l|}{\textbf{0.995}} &
          \textbf{0.122} &
          \textbf{0.073} &
          \textbf{0.426} &
          \textbf{0.155} \\
        \multirow{-3}{*}{\begin{tabular}[c]{@{}l@{}}PKT~\cite{Passalis2018LearningTransfer} \\     \textit{\scriptsize ECCV 2018}\end{tabular}} &
          \textit{Improvement} &
          \cellcolor[HTML]{F5FFF5}\textit{0.29\%} &
          \cellcolor[HTML]{FCFFFC}\textit{0.10\%} &
          \multicolumn{1}{l|}{\cellcolor[HTML]{FFFFFF}\textit{0.00\%}} &
          \cellcolor[HTML]{D3FFD3}\textit{1.22\%} &
          \cellcolor[HTML]{99FF99}\textit{2.80\%} &
          \cellcolor[HTML]{E1FFE1}\textit{0.84\%} &
          \cellcolor[HTML]{EAFFEA}\textit{0.58\%} \\ \midrule
         &
          Traditional &
          0.835 &
          0.973 &
          \multicolumn{1}{l|}{0.995} &
          0.128 &
          0.079 &
          0.446 &
          0.162 \\
         &
          Inverted (Ours) &
          \textbf{0.849} &
          \textbf{0.976} &
          \multicolumn{1}{l|}{\textbf{0.996}} &
          \textbf{0.124} &
          \textbf{0.075} &
          \textbf{0.432} &
          \textbf{0.157} \\
        \multirow{-3}{*}{\begin{tabular}[c]{@{}l@{}}Ensemble~\cite{Chen2022ImprovedEnsemble} \\     \textit{\scriptsize NeurIPS 2022}\end{tabular}} &
          \textit{Improvement} &
          \cellcolor[HTML]{C0FFC0}\textit{1.74\%} &
          \cellcolor[HTML]{F6FFF6}\textit{0.26\%} &
          \multicolumn{1}{l|}{\cellcolor[HTML]{FDFFFD}\textit{0.06\%}} &
          \cellcolor[HTML]{9BFF9B}\textit{2.75\%} &
          \cellcolor[HTML]{4BFF4B}\textit{4.96\%} &
          \cellcolor[HTML]{91FF91}\textit{3.03\%} &
          \cellcolor[HTML]{84FF84}\textit{3.39\%} \\
        \bottomrule
    \end{tabular}
    \vspace{1em}
    \caption{\textbf{Randomly-initialised teacher $\rightarrow$ Depth student (largest task gap).} Our inverted projection produces significant improvement. \textit{Improvement} is \% change using our inverted projection over using the traditional projection. See section \ref{sec:app:model_details} for model details. Baseline $\pm$ figures are variance from 3 runs.}
    \label{tab:supp:full-depth-table:random-teacher}
\end{table}
    
    Each table shows a single teacher/student task pair, and compares four different knowledge distillation methods when using both the traditional projection and our inverted projection, as well as including a percentage \textit{Improvement} showing the difference in performance when using our inverted projection compared to the traditional projection.

    % \newpage
    Table \ref{tab:supp:full-depth-table:depth-teacher} shows results using a depth estimation teacher. As the teacher and student tasks are identical and the task-specific features in the teacher are desired for the student model, the traditional projection produces a greater performance improvement than our inverted projection.
    
    Table \ref{tab:supp:full-depth-table:insseg-teacher} shows results using an instance segmentation teacher. Instance segmentation produces both semantic labels and instance labels, and the semantic masks and labels are known to be useful for depth estimation (see section \ref{sec:related_work}), so while the teacher and student tasks are different, they are similar to one another. Therefore, we see that the traditional projection still outperforms our inverted projection in most cases, as expected.
    
    Table \ref{tab:supp:full-depth-table:class-teacher} shows results with a classification teacher. This is a cross-task setup: classification is relatively unrelated to monocular depth estimation. As a result, it can be seen that our inverted projection outperforms the traditional projection.
    
    Table \ref{tab:supp:full-depth-table:random-teacher} shows results with a randomly-initialised and frozen teacher model. The randomly-initialised teacher does not contain any task-specific knowledge whatsoever, and therefore the task-gap between the teacher and the student model is maximised. As this is the most cross-task setting, our inverted projection performs the best in comparison to the traditional projection, as it is only our inverted projection that is able to successfully discard the confounding features present in the randomly-initialised teacher.

    \input{figures/qualitative_figures}    

    We also provide qualitative examples using same-task, similar-task, and randomly-initialised teachers on a different depth estimation student, shown in figure \ref{fig:qualitative-different-teachers}. In all cases, we are able to obtain qualitatively good performance.

\subsection{Model details}
\label{sec:app:model_details}
    This section details the different student and teacher architectures used for our experiments.

    \subsubsection{Depth estimation}
    \label{sec:app:depth_est_models}
        \paragraph{Teacher models:}
            The teacher models used for depth estimation are:
            \begin{itemize}
                \item 
                    \textbf{Depth teacher}: SwinV2-B \cite{liu_swin_2022} pretrained on NYUv2 as part of the All In Tokens \cite{ning_all_2023} framework.
                    \footnote{\url{https://msravcghub.blob.core.windows.net/ait-release/checkpoint/ait\_depth\_swinv2b\_ar.pth}},
                    available from the official AiT repository\footnote{\url{https://github.com/SwinTransformer/AiT}}.
                \item 
                    \textbf{Instance segmentation teacher}: SwinV2-B pretrained on COCO \cite{Lin2014MicrosoftContext} as part of the All In Tokens framework.
                \item 
                    \textbf{Classification teacher}: ViT-B-16 pretrained on ImageNet-1K, available from the torchvision model hub\footnote{\label{footnote:torchvision-models}\url{https://pytorch.org/vision/stable/models.html}}.
            \end{itemize}

        \paragraph{Student Models:}
        \label{sec:app:depth-student-models}
            The depth estimation students used have one of three backbones:
            \begin{itemize}
                \item MobilenetV2 \cite{Fox2018MobileNetV2:Bottlenecks}: In our experiments, we use a width multiplier of 0.5.
                \item EfficientNet-B0 \cite{tan_efficientnet_2019}.
                \item ResNet-50 \cite{He2015ResNetRecognition}.
            \end{itemize}
            The decoders used are (names in \texttt{this font}):
            \begin{itemize}
                \item \texttt{Decoder}:
                    Conv1x1, then 6 blocks of (LeakyReLU + Conv3x3 + LeakyReLU + Conv3x3). At the input to each of the 6 blocks, an incoming skip connection from the encoder is bilinearly upsampled to match the feature resolution, then concatenated to the features.
                \item \texttt{Decoder\_dl2}:
                    The same as \texttt{Decoder}, except the second Conv3x3 in each block is replaced with a depthwise convolution to reduce parameters.
                \item \texttt{ULightDecoder\_skip\_4b}:
                    Conv1x1, then 4 blocks of (LeakyReLU + Conv3x3). As in the other decoders, each block receives features from an incoming skip connection, which are upsampled to match the feature resolution and then concatenated.
            \end{itemize}

    \subsubsection{Semantic segmentation}
        \paragraph{Teacher models:}
            The teacher models used for semantic segmentation are:
            \begin{itemize}
                \item Segmentation teacher:
                    A DeepLab-V3 \cite{chen_rethinking_2017} with a ResNet-50 backbone, pretrained on a subset of MSCOCO that uses only the 20 categories present in the Pascal VOC dataset. Model and checkpoint loaded from torchvision model hub\footnotemark[\getrefnumber{footnote:torchvision-models}].
                \item Classification teacher: 
                    ResNet-50 \cite{He2015ResNetRecognition} pretrained on ImageNet-1K. Model and checkpoint loaded from torchvision model hub\footnotemark[\getrefnumber{footnote:torchvision-models}].
            \end{itemize}
        \paragraph{Student model:}
            The student model used for semantic segmentation was a DeepLabV3 \cite{chen_deeplab:_2017} with a ResNet50 backbone that is pretrained on ImageNet-1K. The pretrained weights were sourced from the torchvision model hub\footnotemark[\getrefnumber{footnote:torchvision-models}].

    \subsubsection{Satellite-to-map and Colorization}
        We use the same teacher models described in section \ref{sec:app:depth_est_models}. For the student models on the satellite-to-map experiments, we use a CycleGAN, while for the colorization experiments we use a Pix2Pix model. This Pix2Pix model follows a standard UNet-like architecture with batch norm layers.
\subsection{Task losses}
\label{sec:app:loss-functions}
    In addition to the projection loss $\mathcal{L}_{distill}$, each student is trained with a task-specific loss $\mathcal{L}_{task}$ to supervise its output. The task and projection loss components are weighted equally, as in equation \ref{eq:total_loss}.

    The depth task loss function used is a variant of the Scale-Invariant Log-Loss (SILog), first proposed by \cite{eigen_depth_2014} and modified by \cite{bhat_adabins_2020}:
        \begin{equation}
        \label{eq:depth-loss}
        \mathcal{L}_{SILog} = 10 \sqrt{\frac{1}{K}\displaystyle\sum^K_{i = 1} g_{i}^2 + \frac{0.15}{K^2}\left(\displaystyle\sum^K_{i = 1} g_{i}\right)^2}
    \end{equation}
    where ground-truth and predicted depth values for pixel $i$ are given as $d^*_i$ and $d_i$ respectively, $g_{i} = log(d_{i}) - log(d^*_{i})$ and $K$ is the total number of pixels with valid depth values.
    Semantic segmentation students are trained with a pixelwise cross-entropy loss.
    For the colourization task we use the vanilla GAN loss\cite{Goodfellow2014GenerativeNetworks} in addition to an L1 loss with a weighting of $100.0$. For the satellite-to-map translation we use the cyclic consistency loss described in the original CycleGAN paper~\cite{Zhu2017UnpairedNetworks}.

\subsection{Evaluation metrics}
\label{sec:app:metrics}
    \textbf{Monocular depth estimation.} We use the metrics defined in~\cite{eigen_depth_2014}: 
    \begin{itemize}
        \item Abs relative difference (Abs): $\frac{1}{T}\sum_{i=1}^{T} \frac{|d_i - d_i^*|}{d_i^*}$, 
        \item Squared relative difference (Sq): $\frac{1}{T}\sum_{i=1}^{T} \frac{||d_i - d_i^*||^2}{d_i^*}$, 
        \item RMSE (RMS): $\sqrt{\frac{1}{T}\sum_{i=0}^{T}\|d_i - d_i^*\|^2}$, 
        \item Log RMSE (RMSL): $\sqrt{\frac{1}{T}\sum_{i=0}^{T}\|log(d_i) - log(d_i^*)\|^2}$, 
        \item The threshold accuracy $\delta_n$: \(\%\) of \(d_i\) s.t. $max(\frac{d_i}{d_i^*}, \frac{d_i^*}{d_i}) = \delta < thr$, where $\delta_n$ denotes that $thr = 1.25^n$ (we use $n \in \{1, 2, 3\}$). $T$ denotes the total number of valid pixels in the ground truth depth map. $d_i$ and $d_i^*$ represent the predicted and ground-truth depth values at pixel $i$ respectively.
    \end{itemize}
\subsection{Datasets}
\label{sec:app:datasets}
    For semantic segmentation students, we use the ADE20K Scene Parsing dataset \cite{zhou_scene_2017}, a 150-class subset of the full ADE20K dataset. It contains 20210 training images and 2000 testing images from a variety of indoor and outdoor scenes.

    For depth estimation students, the NYUv2 dataset \cite{silberman_indoor_2012} is used, an indoor monocular depth estimation dataset containing 24231 training 654 test examples. Students are trained for 25 epochs.

    For image colorization and satellite-to-map translation, we use the CMP Facades \cite{tylecek_spatial_2013} and Maps datasets used in Pix2Pix \cite{isola_image--image_2018}, both of which are available from \url{https://efrosgans.eecs.berkeley.edu/pix2pix/datasets/}. The Maps dataset was scraped from Google Maps by the Pix2Pix authors.
% \subsection{Training details}
% \label{sec:app:training-details}
\subsection{Hyperparameters}
\label{sec:app:training-details}
\vspace{0.5em}\textbf{Monocular depth estimation.} Depth estimation students were trained for 25 epochs using the AdamW optimizer with a learning rate of 2e-4 and weight decay of 0.05. The OneCycle learning rate scheduler was used \cite{smith_super-convergence_2018} with the maximum learning rate set to 2e-4. The batch size was set to 16.

\vspace{0.5em}\noindent\textbf{Semantic segmentation.} Semantic segmentation students were trained for 80 epochs using the AdamW optimizer with a learning rate of 5e-3 and weight decay of 1e-2. The OneCycle learning rate scheduler was used, with the maximum learning rate set to 5e-3. The batch size was set to 20.

\vspace{0.5em}\noindent\textbf{Image-to-image translation (satellite-to-map, colorization).} Each model for both of these tasks are trained for 200 epochs using the AdamW optimizer with a learning rate of 2e-4. We keep the initial learning rate for the first 100 epochs and then linearly decay the rate to zero over the next 100 epochs with a batch size of 8.

\subsection{Linear mapping between task spaces}
\label{sec:subsec:linear-mapping-between}

\begin{figure}
    \centering
    \subfigure[Input Image]{\hspace{.3\textwidth}}
    \subfigure[Predicted Depth]{\hspace{.3\textwidth}}
    
    \subfigure{\includegraphics[width=0.3\textwidth]{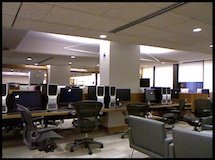}}
    \subfigure{\includegraphics[width=0.3\textwidth]{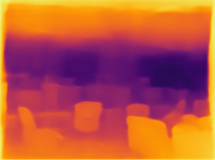}}
    
    \subfigure{\includegraphics[width=0.3\textwidth]{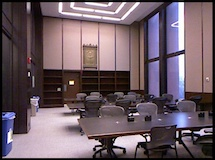}}
    \subfigure{\includegraphics[width=0.3\textwidth]{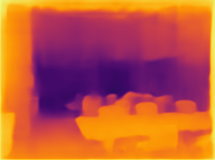}}
    \vspace{1em}
    \caption{\textbf{Qualitative results using a frozen segmentation encoder and frozen depth decoder.} With only a learned linear projection, features from the semantic segmentation task can be made immediately useful for depth.}
    \label{fig:qualitative_toy_experiment}
\end{figure}

In performing cross-task distillation, we assume there is an overlap in information in the representation spaces across different tasks, following both the work in the literature and intuition (see section \ref{sec:related_work}). 
\cite{merullo_linearly_2022} demonstrated the existence of a learnable linear mapping between text and image features. Concurrently, research has shown that linear projections are very effective for knowledge distillation\cite{Chen2022ImprovedEnsemble, miles2024understanding}. However, a natural unification of these two settings has not been explored.

We experimentally verify the validity of this assumption with a simple toy scenario, in which a frozen encoder pretrained on instance segmentation is connected via a learnable linear projection to a frozen decoder pretrained for depth estimation. Example qualitative results in figure \ref{fig:qualitative_toy_experiment} show that the linearly projected cross-task features can be successfully utilized to generate a coherent output, despite both models being frozen. In fact, by only training the linear projector between these two frozen models, we can attain $0.504$ RMSE on NYUv2. This result indicates that a significant portion of the information contained in the instance segmentation features are closely related to the depth estimation task. We conduct additional experiments projecting between various other task representation spaces.
These results indicate that cross-task distillation using linear projection is a promising approach for leveraging shared information between specific pairs of tasks, and further motivate our work.
\subsection{Training Dynamics of the Inverted Projector}
\label{sec:subsec:eigplots_section}

    \input{figures/SV_evolution_graphs} %
    
    By observing the singular value spectrum of the projector weights and how they evolve over the course of training, we are able to provide further insight into the role of our novel inverted projection for cross-task distillation, as compared to the traditional projection.
    Figure \ref{fig:eigplots} shows the singular value spectrum of the projector weights throughout the training process of a segmentation student with both similar and different teacher tasks, using either the traditional projection or our novel inverted projection.
    It can be seen that the traditional projection fails to disregard many of the less-dominant singular values, leading to a higher-rank projection in general.
    As discussed in section \ref{sec:subsec:why-does-proj-space-matter}, this is especially detrimental when there is a significant task gap, as it encourages the student to learn task-irrelevant features.
    When the student model is small, this can significantly degrade the target task performance. 
    However, when using our inverted projection, we observe a consistently lower rank across training for all tasks, compared to the traditional projection.
    This is because of the inverted projection's ability to suppress the task-irrelevant singular vectors from the teacher model: while the traditional projection remains consistently high-rank regardless of the dissimilarity of the student and teacher tasks, our inverted projection is able to adapt to discard the increasing quantity of undesirable task-specific knowledge encoded in the increasingly dissimilar teacher features.
\subsection{Different architecture pairs} 
\begin{figure}[t]
    \centering
    \subfigure[Depth $\rightarrow$ Depth]{\includegraphics[width=.32\textwidth]{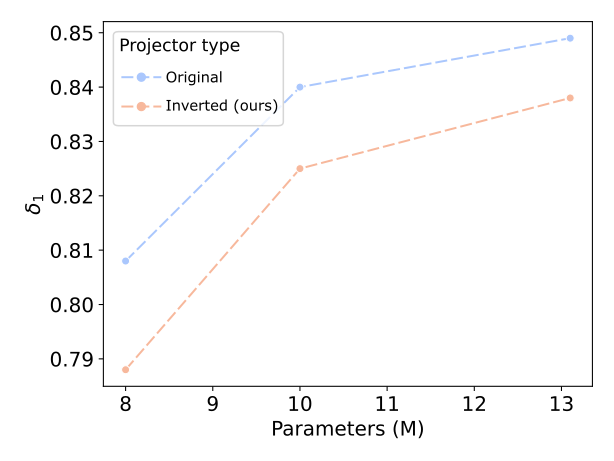}}
    \subfigure[Insseg $\rightarrow$ Depth]{\includegraphics[width=.32\textwidth]{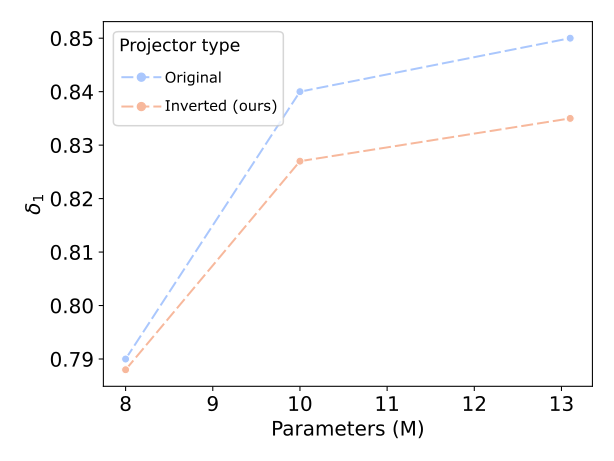}}
    \subfigure[Random $\rightarrow$ Depth]{\includegraphics[width=.32\textwidth]{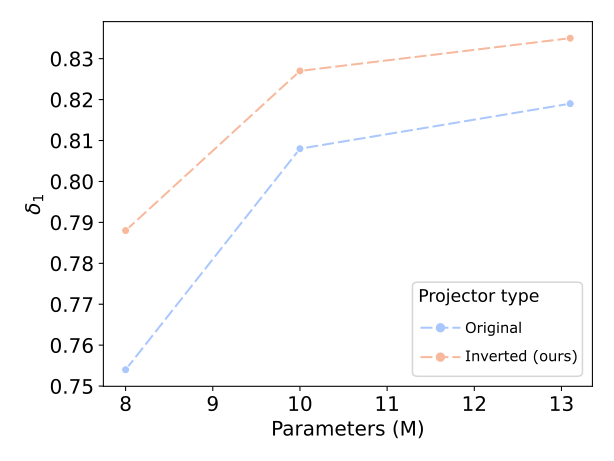}}
    \vspace{1em}
    \caption{\textbf{Comparing performance of different-sized depth students} with both the traditional projection and our novel inverted projection.
    Where there is knowledge to transfer from teacher to student (i.e. the two tasks are similar), the traditional projection performs better, but when the teacher is random, the opposite is true. Only decoder size is varied. A MobileNetV2 \cite{Fox2018MobileNetV2:Bottlenecks} is used as the backbone.}
    \label{fig:params_vs_performances}
\end{figure}

To demonstrate the generality of our proposed inverted projection in various cross-task settings, we perform an ablation across several differently-sized student models with similar and dissimilar task pairs.
Figure \ref{fig:params_vs_performances} shows that the performance drop or improvement is consistent for both the very small and moderately large student models, across different task pairs.
It also mirrors the findings of our previous experiments in sections \ref{sec:subsec:experiments-depth}, \ref{sec:subsec:experiments-seg}, and \ref{sec:subsec:experiments-im2im}, showing that the similarity of the teacher and student tasks matters, and that our novel inverted projection performs best when the two tasks are dissimilar.

\begin{table}[t]
\centering
\scriptsize
\resizebox{1\textwidth}{!}{
\begin{tabularx}{\textwidth}{XX|ccc|ccc}
\toprule
\belowrulesepcolor{mygrey}
\rowcolor{mygrey} \multicolumn{2}{r|}{Student Arch (backbone) $\longrightarrow$} &
  \multicolumn{3}{c|}{EfficientNet-B0 (5.3M)} &
  \multicolumn{3}{c}{ResNet-50 (25.6M)} \\
\rowcolor{mygrey} KD Method &
  Projection type &
  $\delta_1 \uparrow$ &
  Abs. $\downarrow$ &
  RMS $\downarrow$ &
  $\delta_1 \uparrow$ &
  Abs. $\downarrow$ &
  RMS $\downarrow$ \\ 
\aboverulesepcolor{mygrey}  
\midrule
\textit{None (baseline)} &
  \textit{N/A} &
  0.845 &
  0.127 &
  0.440 &
  0.811 &
  0.144 &
  0.480 \\ \midrule
AT~\cite{Zagoruyko2019PayingTransfer} &
  Original &
  0.850 &
  0.125 &
  0.433 &
  0.814 &
  \textbf{0.143} &
  0.477 \\
 &
  Inverted (ours) &
  \textbf{0.853} &
  \textbf{0.123} &
  \textbf{0.430} &
  \textbf{0.816} &
  \textbf{0.143} &
  \textbf{0.475} \\
 &
  \textit{Improvement} &
  \cellcolor[HTML]{F3FFF3}\textit{0.35\%} &
  \cellcolor[HTML]{C5FFC5}\textit{1.61\%} &
  \cellcolor[HTML]{E3FFE3}\textit{0.79\%} &
  \cellcolor[HTML]{F6FFF6}\textit{0.26\%} &
  \cellcolor[HTML]{FAFFFA}\textit{0.14\%} &
  \cellcolor[HTML]{F2FFF2}\textit{0.38\%} \\ \midrule
PKT~\cite{Passalis2018LearningTransfer} &
  Original &
  0.851 &
  0.124 &
  0.432 &
  0.816 &
  0.143 &
  0.473 \\
 &
  Inverted (ours) &
  \textbf{0.853} &
  \textbf{0.123} &
  \textbf{0.431} &
  \textbf{0.821} &
  \textbf{0.141} &
  \textbf{0.470} \\
 &
  \textit{Improvement} &
  \cellcolor[HTML]{F7FFF7}\textit{0.25\%} &
  \cellcolor[HTML]{D1FFD1}\textit{1.29\%} &
  \cellcolor[HTML]{F5FFF5}\textit{0.30\%} &
  \cellcolor[HTML]{E9FFE9}\textit{0.63\%} &
  \cellcolor[HTML]{D4FFD4}\textit{1.19\%} &
  \cellcolor[HTML]{E6FFE6}\textit{0.70\%} \\ \midrule
FitNets~\cite{romero_fitnets_2015} &
  Original &
  0.845 &
  0.125 &
  0.439 &
  0.812 &
  0.145 &
  0.480 \\
 &
  Inverted (ours) &
  \textbf{0.850} &
  \textbf{0.124} &
  \textbf{0.434} &
  \textbf{0.813} &
  \textbf{0.142} &
  \textbf{0.476} \\
 &
  \textit{Improvement} &
  \cellcolor[HTML]{EDFFED}\textit{0.50\%} &
  \cellcolor[HTML]{ECFFEC}\textit{0.53\%} &
  \cellcolor[HTML]{CFFFCF}\textit{1.34\%} &
  \cellcolor[HTML]{FAFFFA}\textit{0.16\%} &
  \cellcolor[HTML]{B9FFB9}\textit{1.93\%} &
  \cellcolor[HTML]{E3FFE3}\textit{0.77\%} \\ \bottomrule
\end{tabularx}%
}
\vspace{1em}
\caption{\textbf{Comparisons with different architecture pairs.} All experiments perform cross-task distillation from a classification teacher to a depth estimation student. The inverted projection is effective across various student model sizes and with different KD methods in this cross-task setting.}
\label{tab:rebuttal:enetb0-rn50-class2depth}
\end{table}

Table \ref{tab:rebuttal:enetb0-rn50-class2depth} shows results distilling from a classification teacher to a depth student using two student backbones of significantly-different sizes: an EfficientNet-B0 (5.3M params) and a ResNet-50 (25.6M params). These students are chosen to illustrate both a small and a large capacity gap between the student and teacher models.
Three different KD methods are used. Our inverted projector outperforms the traditional projector across all metrics for all three KD methods and both student backbone architectures in this cross-task setting, thus demonstrating the generality of our inverted projector for a variety of practical KD settings.

\subsection{Teacher-Free Distillation: Results}

\begin{table}
    \centering
    \footnotesize
    \begin{tabular}{lccc}
        \toprule
        \belowrulesepcolor{mygrey}
        \rowcolor{mygrey} Method & RMS $\downarrow$ & Abs $\downarrow$ & $\delta_1$ $\uparrow$ \\
        \aboverulesepcolor{mygrey}
        \midrule
        \textit{(Baseline) AiT (SwinV2-B) \cite{ning_all_2023}} & \textit{0.365}            & \textit{0.105}            & \textit{0.907}                 \\
        \midrule
         $\mathcal{L}_{spectral}$ $(r = 1)$              & 0.352            & 0.105            & 0.902                 \\
         $\mathcal{L}_{spectral}$ $(r = 2)$              & \textbf{0.340}   & \textbf{0.096}   & \textbf{0.914}        \\
         $\mathcal{L}_{spectral}$ $(r = 4)$              & 0.349            & 0.099            & 0.911                 \\
         $\mathcal{L}_{spectral}$ $(r = 8)$              & 0.344            & \textbf{0.096}   & 0.910                 \\
         $\mathcal{L}_{spectral}$ $(r = 16)$             & 0.348            & 0.098            & 0.912                 \\
         $\mathcal{L}_{spectral}$ $(r = 32)$             & 0.347            & 0.100            & 0.909                 \\
        \bottomrule
    \end{tabular}
    \vspace{1em}
    \caption{\textbf{Teacher-free distillation} using our spectral regularisation loss on the NYUv2 dataset using AiT \cite{ning_all_2023} on a SwinV2-b base. The regularisation loss is generally robust to different values of $r$, with $r = 2$ being optimal.
    }
    \label{tab:manual-reg-ait}
\end{table}

Table \ref{tab:manual-reg-ait} shows the performance of the teacher-free distillation strategy detailed in section \ref{sec:subsec:experiments-ablation-study-teacher-free-backbones} using different ranks, when applied to a depth estimation setup. A higher value of $r$ uses more of the available principal components to reconstruct the features. The optimal value is found to be when $r=2$.
\subsection{Choice of CycleGAN representation}
\label{sec:choice_of_representation}
In the encoder-decoder setup, there is a natural choice for the representation to be used as the distillation loss: the representation at the output of the encoder. However, when dealing with different architectures, the decision is less obvious and can significantly impact the efficacy of the distillation process itself. 
The CycleGAN architecture consists of a discriminator and two separate encoder-decoder models (generators), which we denote here as $G_A(\cdot)$ and $G_B(\cdot)$. The first of these, $G_A(\cdot)$, attempts to generate an image from the input $\mathbf{x}$ that will fool the discriminator, and the second, $G_B(\cdot)$, maps the output of $G_A(\cdot)$ back to the source domain.

Both $G_A(\cdot)$ and $G_B(\cdot)$ are encoder-decoders, and we represent the intermediate features as $G_{A_E}(\cdot)$ and $G_{B_E}(\cdot)$ for each respectively. We trialled the use of each set of features, the results of which are shown in table \ref{tab:choice_repr_distill}, and found a significant improvement when using the representation from the generator that maps back to the source domain:  $\mathbf{Z}_s = G_{B_E}(G_A(\mathbf{x}))$. Therefore, the features from the second generator $G_B(\cdot)$ are those used for feature distillation in our main CycleGAN experiments.

\begin{table}
    \centering
    \begin{tabular}[t]{llll}
        \toprule
        Teacher Task & Position & PSNR $\uparrow$ & FID $\downarrow$ \\
        \midrule
        KeyPoint Det.& $\mathbf{Z}_s = G_{B_E}(G_A(x))$ & \textbf{35.77} & \textbf{68.77} \\
        KeyPoint Det.& $\mathbf{Z}_s = G_{A_E}(x)$ & 34.97 & 70.28 \\
        \midrule
        Image Classif.& $\mathbf{Z}_s = G_{B_E}(G_A(x))$ & \textbf{36.28} & \textbf{59.86} \\
        Image Classif.& $\mathbf{Z}_s = G_{A_E}(x)$ & 35.94 & 66.98 \\
        \bottomrule
    \end{tabular}
    \vspace{1em}
    \caption{\textbf{Choice of representation} for the distillation loss: either using features from the first generator $G_A(\cdot)$ that generates the synthetic image, or using features from the second generator $G_B(\cdot)$ that maps the synthetic image back to the input domain.}
    \label{tab:choice_repr_distill}
\end{table}
\subsection{Analysis of Feature Distillation Loss}
\label{sec:novel-analysis-fd}

This section describes the full analysis of the loss function $\mathcal{L}_{distill}$ detailed in section \ref{sec:subsec:decoupled} that leads to it breaking into the knowledge transfer component and the regularisation component in equation \ref{eq:decoupled_loss}.

\subsection{Setup and Definitions}
    We begin by describing our setup. A teacher model, $T$, and a student model, $S$, both take an identical input to produce the teacher and student features, $\mathbf{Z}_t \in \mathbb{R}^{b\times d_t}$ and $\mathbf{Z}_s \in \mathbb{R}^{b\times d_s}$ respectively, where $d_t$ and $d_s$ are the sizes of the feature dimensions for the teacher and student models respectively, and $b$ is the batch size.
    We also define the inverted projection matrix between the teacher and student feature spaces
    $\mathbf{P}$.
    The corresponding projected features would be given by $\bar{\mathbf{Z}}_t = \mathbf{Z}_t\mathbf{P} \in \mathbb{R}^{b \times d_s}$.
    The rank $r$ for each of these is bounded by:
    \begin{align}
        r_s &= Rank(\mathbf{Z}_s) \leq \min(b, d_s) \\
        r_t &= Rank(\mathbf{Z}_t) \leq \min(b, d_t) \\
        r_{p} &= Rank(\mathbf{P}) \leq \min(d_t, d_s) \\
        \bar{r}_t &= Rank(\mathbf{Z}_t\mathbf{P}) \leq \min(r_t, r_{p}) \\
            & \leq \min(\min(b, d_t), \min(d_t, d_s)),
    \end{align}
    with the latter being due to the fact that $Rank(\mathbf{A}\mathbf{B}) \leq \min(Rank(\mathbf{A}), Rank(\mathbf{B}))$.

\subsection{Understanding the Inverted Projection}
    We demonstrate using our inverted projection.
    The feature distillation loss function is given by:
    \begin{equation}
        \mathcal{L}_{distill} = \lpnormv{\bar{\mathbf{Z}}_t - \mathbf{Z}_s}_2 = \lpnormv{\mathbf{Z}_t\mathbf{P} - \mathbf{Z}_s}_2
    \end{equation}

    Taking the singular value decomposition of each of these gives $\bar{\mathbf{Z}}_t = \bar{\mathbf{U}}\bar{\pmb{\Sigma}} \bar{\mathbf{V}}^T$ and
    $\mathbf{Z}_s = \mathbf{U}\pmb{\Sigma} \mathbf{V}^T$.
    Using the rank definitions mentioned previously, we can express these as sums of products of the singular values and their corresponding singular vectors, i.e.
    \begin{align}    
        \bar{\mathbf{Z}}_t &= \mathbf{Z}_t\mathbf{P} = \sum_{i=1}^{\bar{r}_t} \bar{\sigma}_i\bar{\mathbf{u}}_i\bar{\mathbf{v}}_i \\
        \mathbf{Z}_s &= \sum_{i=1}^{r_s}\sigma_i\mathbf{u}_i\mathbf{v}_i
    \end{align}
    where $\bar{\pmb{\sigma}} \in \Real^{\bar{r}_t}$ and
        $\pmb{\sigma} \in \Real^{r_s}$ 
    denote the columns of $\bar{\pmb{\Sigma}}$ and $\pmb{\Sigma}$ respectively,
    $\bar{\mathbf{u}} \in \Real^{b \times \bar{r_t}}$
        and $\mathbf{u} \in \Real^{b \times r_s}$ 
    the columns of $\bar{\mathbf{U}}$ and $\mathbf{U}$, 
    and $\bar{\mathbf{v}}\in \Real^{\bar{r}_t \times d_s}$, 
        and $\mathbf{v}\in \Real^{r_s \times d_s}$
    the columns of $\bar{\mathbf{V}}$ and $\mathbf{V}$. The feature distillation loss can be rewritten as:
    \begin{align}
        \mathcal{L}_{distill} &= \lpnormv{\bar{\mathbf{Z}}_t - \mathbf{Z}_s}_2 \\
        &= 
        \color{r2d}
        \underbrace{\lpnormv{\sum_{i=1}^{\bar{r}_t} \bar{\sigma}_i\bar{\mathbf{u}}_i\bar{\mathbf{v}}_i - \sum_{i=1}^{r_s}\sigma_i\mathbf{u}_i\mathbf{v}_i}_2}_{\text{knowledge transfer \textbf{only}}} && \textit{1. Same-task}
        \label{eq:fdanalysis-uncombined_sum}
    \end{align}

    The rank of the inverted projection matrix dictates how the upper bound on the loss can be decomposed into a knowledge transfer component and a regularisation component. We empirically find that $\mathbf{P}$ works out to be lower-rank in the cross-task setting (see section \ref{sec:subsec:eigplots_section}), and so $r_s > \bar{r}_t$. 
    This observation allows us to merge the sum in equation \ref{eq:fdanalysis-uncombined_sum} such that every one of the $\bar{r}_t$ projected teacher singular values is compared to a student singular value, with the remaining $r_s - \bar{r}_t$ student singular values forming the regularisation term:
    \begin{small}
        \begin{align}
            \mathcal{L}_{distill} &= \lpnormv{
                \sum_{i=1}^{\bar{r}_t}( \bar{\sigma}_i\bar{\mathbf{u}}_i\bar{\mathbf{v}}_i^T - \sigma_i\mathbf{u}_i\mathbf{v}_i) + 
                \sum_{i=\bar{r}_t+1}^{r_s}\sigma_i\mathbf{u}_i\mathbf{v}_i
                }_2 \nonumber \\
            & \leq \begingroup
            \color{r2d}
                \underbrace{\lpnormv{\sum_{i=1}^{\bar{r}_t}
                    \bar{\sigma}_i{\bar{\mathbf{u}}_i\bar{\mathbf{v}}_i^T -
                    \sigma_i \mathbf{u}_i \mathbf{v}_i^T
                }}_2}_{\text{knowledge transfer}} 
            \endgroup + \begingroup
            \color{s2d}
                \underbrace{\lpnormv{\sum_{i=\bar{r}_t+1}^{r_s} \sigma_{i}\mathbf{u}_{i}\mathbf{v}_{i}^T}_2}_{\text{student regularisation}}
        \endgroup && \textit{2. Cross-task}
        \label{eq:fdanalysis-two-term-loss-bound}
        \end{align}
    \end{small}
    This shows that, under the cross-task setting, the feature distillation contains both a knowledge transfer component (which incorporates information from the teacher model) and a regularisation component (which acts upon the student model).

%%%%%%%%%%%%%%%%%%
%% Included for supplementary - remove if using as appendix.
% {\small
% \bibliographystyle{splncs04}
% \bibliography{references, refs, references-da}
% }
\bibliography{references, refs, references-da}
