# Supplementary material for: Learning to Project for Cross-Task Knowledge Distillation
Source: arXiv:2403.14494 source file (2024-11-27)
Supplement: Supplementary file 2 [file prelim-enc-dec.tex]

\section{Preliminary experiments (Encoder-Encoder and Encoder-Decoder)}
    As a preliminary experiment to ascertain the degree to which a linear mapping is able to "translate" one feature space to another between different tasks, we undertook preliminary experiments: in the first, we learn to map between two frozen and different encoders trained for separate tasks, and in the second we learn a mapping from a frozen encoder for one task to a frozen decoder for another task.
    
    The pipeline for the frozen encoder to frozen encoder setup is shown in figure \ref{fig:enc-enc}. In this setup, two frozen encoders, each pretrained on different tasks, are used to encode the same input image. A linear projection is then applied to map one set of features into the other feature space, and a loss is applied between the two sets of features in the common feature space. This experiment was used to verify that a mapping between the two feature spaces may be learned, which we verified by observing that the loss between the two sets of features (one projected, one not) decreases over the course of training.
    We observed that the projection loss consistently tends towards zero, indicating a significant information overlap between the representation spaces. We examined the projection of depth, instance segmentation, and classification tasks onto the depth space. The projection loss (cosine similarity) for each of these experiments was within $\pm 0.002$ of each other after training for more than 100 epochs.
    Our findings support the efficacy of this projection approach, highlighting its potential for facilitating cross-task knowledge distillation. 

    The pipeline for the frozen encoder to frozen decoder setup is shown in figure \ref{fig:enc-dec}. In this setup, a frozen encoder that is pretrained on one task is connected (via a linear projection) to the frozen decoder from a model trained on a different task. We observe that, despite only the linear projection being learned, the features from task A (instance segmentation in our case) can be made immediately useful for task B (depth estimation), verifying that the features from the instance segmentation task contain information that pertains to depth estimation. This result is discussed in section 3.1 of the main paper.

    \begin{figure}
        \centering
        \includegraphics[width=0.7\linewidth]{figures/enc-enc.pdf}
        \caption{\textbf{The encoder-to-encoder setup.} To verify that there exists a (somewhat) linear mapping between different task feature spaces, the encoders of two pretrained model are used, and a linear projection of one model's features to the other model's feature space is learned.
        }
        \label{fig:enc-enc}
    \end{figure}
    \begin{figure}
        \centering
        \includegraphics[width=0.8\linewidth]{figures/enc-dec.pdf}
        \caption{\textbf{The encoder-to-decoder setup.} To confirm that features for one task contain useful information for another task, this setup is used. A frozen encoder and frozen decoder, trained for tasks A and B respectively, are connected in feature space with the learnable linear projection $\mathbf{P}_{A \rightarrow B}$.}
        \label{fig:enc-dec}
    \end{figure}
