# Supplementary material for: Learning to Project for Cross-Task Knowledge Distillation
Source: arXiv:2403.14494 source file (2024-11-27)
Supplement: Supplementary file 3 [file FD_analysis.tex]

\subsection{Analysis of Feature Distillation Loss}
\label{sec:novel-analysis-fd}

This section describes the full analysis of the loss function $\mathcal{L}_{distill}$ detailed in section \ref{sec:subsec:decoupled} that leads to it breaking into the knowledge transfer component and the regularisation component in equation \ref{eq:decoupled_loss}.

\subsection{Setup and Definitions}
    We begin by describing our setup. A teacher model, $T$, and a student model, $S$, both take an identical input to produce the teacher and student features, $\mathbf{Z}_t \in \mathbb{R}^{b\times d_t}$ and $\mathbf{Z}_s \in \mathbb{R}^{b\times d_s}$ respectively, where $d_t$ and $d_s$ are the sizes of the feature dimensions for the teacher and student models respectively, and $b$ is the batch size.
    We also define the inverted projection matrix between the teacher and student feature spaces
    $\mathbf{P}$.
    The corresponding projected features would be given by $\bar{\mathbf{Z}}_t = \mathbf{Z}_t\mathbf{P} \in \mathbb{R}^{b \times d_s}$.
    The rank $r$ for each of these is bounded by:
    \begin{align}
        r_s &= Rank(\mathbf{Z}_s) \leq \min(b, d_s) \\
        r_t &= Rank(\mathbf{Z}_t) \leq \min(b, d_t) \\
        r_{p} &= Rank(\mathbf{P}) \leq \min(d_t, d_s) \\
        \bar{r}_t &= Rank(\mathbf{Z}_t\mathbf{P}) \leq \min(r_t, r_{p}) \\
            & \leq \min(\min(b, d_t), \min(d_t, d_s)),
    \end{align}
    with the latter being due to the fact that $Rank(\mathbf{A}\mathbf{B}) \leq \min(Rank(\mathbf{A}), Rank(\mathbf{B}))$.

\subsection{Understanding the Inverted Projection}
    We demonstrate using our inverted projection.
    The feature distillation loss function is given by:
    \begin{equation}
        \mathcal{L}_{distill} = \lpnormv{\bar{\mathbf{Z}}_t - \mathbf{Z}_s}_2 = \lpnormv{\mathbf{Z}_t\mathbf{P} - \mathbf{Z}_s}_2
    \end{equation}

    Taking the singular value decomposition of each of these gives $\bar{\mathbf{Z}}_t = \bar{\mathbf{U}}\bar{\pmb{\Sigma}} \bar{\mathbf{V}}^T$ and
    $\mathbf{Z}_s = \mathbf{U}\pmb{\Sigma} \mathbf{V}^T$.
    Using the rank definitions mentioned previously, we can express these as sums of products of the singular values and their corresponding singular vectors, i.e.
    \begin{align}    
        \bar{\mathbf{Z}}_t &= \mathbf{Z}_t\mathbf{P} = \sum_{i=1}^{\bar{r}_t} \bar{\sigma}_i\bar{\mathbf{u}}_i\bar{\mathbf{v}}_i \\
        \mathbf{Z}_s &= \sum_{i=1}^{r_s}\sigma_i\mathbf{u}_i\mathbf{v}_i
    \end{align}
    where $\bar{\pmb{\sigma}} \in \Real^{\bar{r}_t}$ and
        $\pmb{\sigma} \in \Real^{r_s}$ 
    denote the columns of $\bar{\pmb{\Sigma}}$ and $\pmb{\Sigma}$ respectively,
    $\bar{\mathbf{u}} \in \Real^{b \times \bar{r_t}}$
        and $\mathbf{u} \in \Real^{b \times r_s}$ 
    the columns of $\bar{\mathbf{U}}$ and $\mathbf{U}$, 
    and $\bar{\mathbf{v}}\in \Real^{\bar{r}_t \times d_s}$, 
        and $\mathbf{v}\in \Real^{r_s \times d_s}$
    the columns of $\bar{\mathbf{V}}$ and $\mathbf{V}$. The feature distillation loss can be rewritten as:
    \begin{align}
        \mathcal{L}_{distill} &= \lpnormv{\bar{\mathbf{Z}}_t - \mathbf{Z}_s}_2 \\
        &= 
        \color{r2d}
        \underbrace{\lpnormv{\sum_{i=1}^{\bar{r}_t} \bar{\sigma}_i\bar{\mathbf{u}}_i\bar{\mathbf{v}}_i - \sum_{i=1}^{r_s}\sigma_i\mathbf{u}_i\mathbf{v}_i}_2}_{\text{knowledge transfer \textbf{only}}} && \textit{1. Same-task}
        \label{eq:fdanalysis-uncombined_sum}
    \end{align}

    The rank of the inverted projection matrix dictates how the upper bound on the loss can be decomposed into a knowledge transfer component and a regularisation component. We empirically find that $\mathbf{P}$ works out to be lower-rank in the cross-task setting (see section \ref{sec:subsec:eigplots_section}), and so $r_s > \bar{r}_t$. 
    This observation allows us to merge the sum in equation \ref{eq:fdanalysis-uncombined_sum} such that every one of the $\bar{r}_t$ projected teacher singular values is compared to a student singular value, with the remaining $r_s - \bar{r}_t$ student singular values forming the regularisation term:
    \begin{small}
        \begin{align}
            \mathcal{L}_{distill} &= \lpnormv{
                \sum_{i=1}^{\bar{r}_t}( \bar{\sigma}_i\bar{\mathbf{u}}_i\bar{\mathbf{v}}_i^T - \sigma_i\mathbf{u}_i\mathbf{v}_i) + 
                \sum_{i=\bar{r}_t+1}^{r_s}\sigma_i\mathbf{u}_i\mathbf{v}_i
                }_2 \nonumber \\
            & \leq \begingroup
            \color{r2d}
                \underbrace{\lpnormv{\sum_{i=1}^{\bar{r}_t}
                    \bar{\sigma}_i{\bar{\mathbf{u}}_i\bar{\mathbf{v}}_i^T -
                    \sigma_i \mathbf{u}_i \mathbf{v}_i^T
                }}_2}_{\text{knowledge transfer}} 
            \endgroup + \begingroup
            \color{s2d}
                \underbrace{\lpnormv{\sum_{i=\bar{r}_t+1}^{r_s} \sigma_{i}\mathbf{u}_{i}\mathbf{v}_{i}^T}_2}_{\text{student regularisation}}
        \endgroup && \textit{2. Cross-task}
        \label{eq:fdanalysis-two-term-loss-bound}
        \end{align}
    \end{small}
    This shows that, under the cross-task setting, the feature distillation contains both a knowledge transfer component (which incorporates information from the teacher model) and a regularisation component (which acts upon the student model).
