# Supplementary material for: Learning to Project for Cross-Task Knowledge Distillation
Source: arXiv:2403.14494 source file (2024-11-27)
Supplement: Supplementary file 4 [file choice-of-cyclegan-representation.tex]

\subsection{Choice of CycleGAN representation}
\label{sec:choice_of_representation}
In the encoder-decoder setup, there is a natural choice for the representation to be used as the distillation loss: the representation at the output of the encoder. However, when dealing with different architectures, the decision is less obvious and can significantly impact the efficacy of the distillation process itself. 
The CycleGAN architecture consists of a discriminator and two separate encoder-decoder models (generators), which we denote here as $G_A(\cdot)$ and $G_B(\cdot)$. The first of these, $G_A(\cdot)$, attempts to generate an image from the input $\mathbf{x}$ that will fool the discriminator, and the second, $G_B(\cdot)$, maps the output of $G_A(\cdot)$ back to the source domain.

Both $G_A(\cdot)$ and $G_B(\cdot)$ are encoder-decoders, and we represent the intermediate features as $G_{A_E}(\cdot)$ and $G_{B_E}(\cdot)$ for each respectively. We trialled the use of each set of features, the results of which are shown in table \ref{tab:choice_repr_distill}, and found a significant improvement when using the representation from the generator that maps back to the source domain:  $\mathbf{Z}_s = G_{B_E}(G_A(\mathbf{x}))$. Therefore, the features from the second generator $G_B(\cdot)$ are those used for feature distillation in our main CycleGAN experiments.

\begin{table}
    \centering
    \begin{tabular}[t]{llll}
        \toprule
        Teacher Task & Position & PSNR $\uparrow$ & FID $\downarrow$ \\
        \midrule
        KeyPoint Det.& $\mathbf{Z}_s = G_{B_E}(G_A(x))$ & \textbf{35.77} & \textbf{68.77} \\
        KeyPoint Det.& $\mathbf{Z}_s = G_{A_E}(x)$ & 34.97 & 70.28 \\
        \midrule
        Image Classif.& $\mathbf{Z}_s = G_{B_E}(G_A(x))$ & \textbf{36.28} & \textbf{59.86} \\
        Image Classif.& $\mathbf{Z}_s = G_{A_E}(x)$ & 35.94 & 66.98 \\
        \bottomrule
    \end{tabular}
    \vspace{1em}
    \caption{\textbf{Choice of representation} for the distillation loss: either using features from the first generator $G_A(\cdot)$ that generates the synthetic image, or using features from the second generator $G_B(\cdot)$ that maps the synthetic image back to the input domain.}
    \label{tab:choice_repr_distill}
\end{table}
