# Supplementary material for: Learning to Project for Cross-Task Knowledge Distillation
Source: arXiv:2403.14494 source file (2024-11-27)
Supplement: Supplementary file 5 [file code.tex]

\subsection{Code}
\label{sec:app:code}
    We include our anonymised code in the accompanying .zip file, and will release it publicly upon acceptance. Our codebase is written in Python using PyTorch \cite{paszke_pytorch_2019} and is based on several other codebases:
    \begin{itemize}
        \item \textbf{Monocular depth estimation student:} we build on the codebase of AiT \cite{ning_all_2023}, which is built in turn on MMDetection \cite{mmdetection_contributors_openmmlab_2018}. No license is specified in the original AiT repository. MMDetection is released under the Apache license.
        \item \textbf{Semantic segmentation:} our code builds on the pipeline of \\ \url{github.com/yassouali/pytorch-segmentation} \\(released under MIT license).
        \item \textbf{Image-to-image translation:} our code builds on the official PyTorch implementation of Pix2Pix and CycleGAN (released under the BSD license):\\ \url{github.com/junyanz/pytorch-CycleGAN-and-pix2pix}
    \end{itemize}

    A full README is included in the code release, and includes instructions for setup, evaluation, and training.
