# Supplementary material for: Learning to Project for Cross-Task Knowledge Distillation
Source: arXiv:2403.14494 source file (2024-11-27)
Supplement: Supplementary file 6 [file datasets.tex]

\subsection{Datasets}
\label{sec:app:datasets}
    For semantic segmentation students, we use the ADE20K Scene Parsing dataset \cite{zhou_scene_2017}, a 150-class subset of the full ADE20K dataset. It contains 20210 training images and 2000 testing images from a variety of indoor and outdoor scenes.

    For depth estimation students, the NYUv2 dataset \cite{silberman_indoor_2012} is used, an indoor monocular depth estimation dataset containing 24231 training 654 test examples. Students are trained for 25 epochs.

    For image colorization and satellite-to-map translation, we use the CMP Facades \cite{tylecek_spatial_2013} and Maps datasets used in Pix2Pix \cite{isola_image--image_2018}, both of which are available from \url{https://efrosgans.eecs.berkeley.edu/pix2pix/datasets/}. The Maps dataset was scraped from Google Maps by the Pix2Pix authors.
