# Supplementary material for: Learning to Project for Cross-Task Knowledge Distillation
Source: arXiv:2403.14494 source file (2024-11-27)
Supplement: Supplementary file 7 [file different-arch-pairs.tex]

\subsection{Different architecture pairs} 
\begin{figure}[t]
    \centering
    \subfigure[Depth $\rightarrow$ Depth]{\includegraphics[width=.32\textwidth]{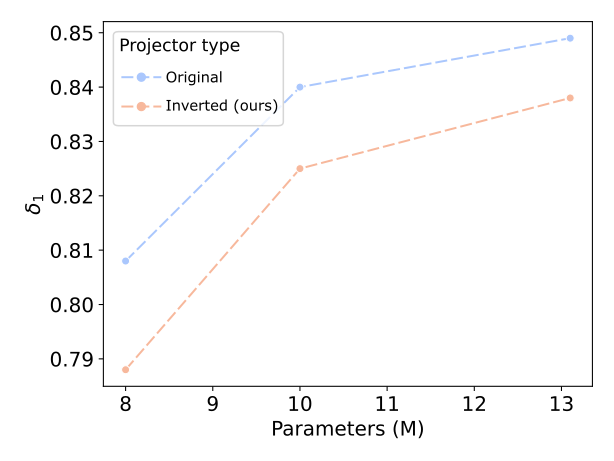}}
    \subfigure[Insseg $\rightarrow$ Depth]{\includegraphics[width=.32\textwidth]{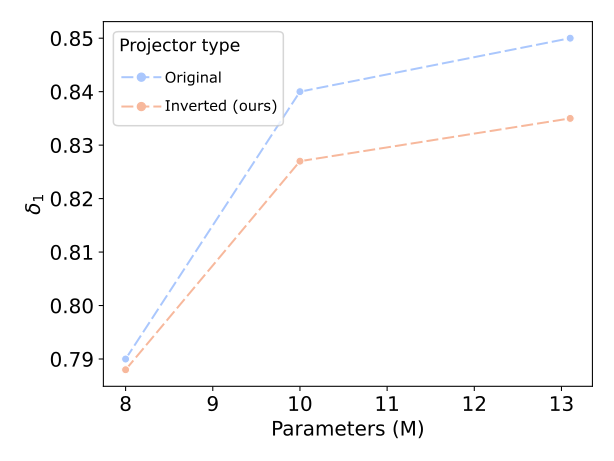}}
    \subfigure[Random $\rightarrow$ Depth]{\includegraphics[width=.32\textwidth]{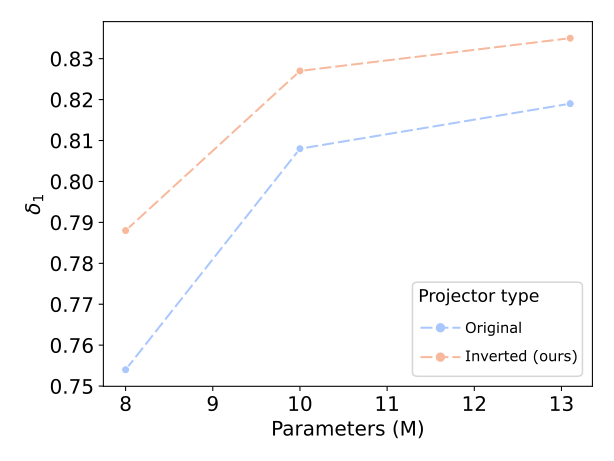}}
    \vspace{1em}
    \caption{\textbf{Comparing performance of different-sized depth students} with both the traditional projection and our novel inverted projection.
    Where there is knowledge to transfer from teacher to student (i.e. the two tasks are similar), the traditional projection performs better, but when the teacher is random, the opposite is true. Only decoder size is varied. A MobileNetV2 \cite{Fox2018MobileNetV2:Bottlenecks} is used as the backbone.}
    \label{fig:params_vs_performances}
\end{figure}

To demonstrate the generality of our proposed inverted projection in various cross-task settings, we perform an ablation across several differently-sized student models with similar and dissimilar task pairs.
Figure \ref{fig:params_vs_performances} shows that the performance drop or improvement is consistent for both the very small and moderately large student models, across different task pairs.
It also mirrors the findings of our previous experiments in sections \ref{sec:subsec:experiments-depth}, \ref{sec:subsec:experiments-seg}, and \ref{sec:subsec:experiments-im2im}, showing that the similarity of the teacher and student tasks matters, and that our novel inverted projection performs best when the two tasks are dissimilar.

\begin{table}[t]
\centering
\scriptsize
\resizebox{1\textwidth}{!}{
\begin{tabularx}{\textwidth}{XX|ccc|ccc}
\toprule
\belowrulesepcolor{mygrey}
\rowcolor{mygrey} \multicolumn{2}{r|}{Student Arch (backbone) $\longrightarrow$} &
  \multicolumn{3}{c|}{EfficientNet-B0 (5.3M)} &
  \multicolumn{3}{c}{ResNet-50 (25.6M)} \\
\rowcolor{mygrey} KD Method &
  Projection type &
  $\delta_1 \uparrow$ &
  Abs. $\downarrow$ &
  RMS $\downarrow$ &
  $\delta_1 \uparrow$ &
  Abs. $\downarrow$ &
  RMS $\downarrow$ \\ 
\aboverulesepcolor{mygrey}  
\midrule
\textit{None (baseline)} &
  \textit{N/A} &
  0.845 &
  0.127 &
  0.440 &
  0.811 &
  0.144 &
  0.480 \\ \midrule
AT~\cite{Zagoruyko2019PayingTransfer} &
  Original &
  0.850 &
  0.125 &
  0.433 &
  0.814 &
  \textbf{0.143} &
  0.477 \\
 &
  Inverted (ours) &
  \textbf{0.853} &
  \textbf{0.123} &
  \textbf{0.430} &
  \textbf{0.816} &
  \textbf{0.143} &
  \textbf{0.475} \\
 &
  \textit{Improvement} &
  \cellcolor[HTML]{F3FFF3}\textit{0.35\%} &
  \cellcolor[HTML]{C5FFC5}\textit{1.61\%} &
  \cellcolor[HTML]{E3FFE3}\textit{0.79\%} &
  \cellcolor[HTML]{F6FFF6}\textit{0.26\%} &
  \cellcolor[HTML]{FAFFFA}\textit{0.14\%} &
  \cellcolor[HTML]{F2FFF2}\textit{0.38\%} \\ \midrule
PKT~\cite{Passalis2018LearningTransfer} &
  Original &
  0.851 &
  0.124 &
  0.432 &
  0.816 &
  0.143 &
  0.473 \\
 &
  Inverted (ours) &
  \textbf{0.853} &
  \textbf{0.123} &
  \textbf{0.431} &
  \textbf{0.821} &
  \textbf{0.141} &
  \textbf{0.470} \\
 &
  \textit{Improvement} &
  \cellcolor[HTML]{F7FFF7}\textit{0.25\%} &
  \cellcolor[HTML]{D1FFD1}\textit{1.29\%} &
  \cellcolor[HTML]{F5FFF5}\textit{0.30\%} &
  \cellcolor[HTML]{E9FFE9}\textit{0.63\%} &
  \cellcolor[HTML]{D4FFD4}\textit{1.19\%} &
  \cellcolor[HTML]{E6FFE6}\textit{0.70\%} \\ \midrule
FitNets~\cite{romero_fitnets_2015} &
  Original &
  0.845 &
  0.125 &
  0.439 &
  0.812 &
  0.145 &
  0.480 \\
 &
  Inverted (ours) &
  \textbf{0.850} &
  \textbf{0.124} &
  \textbf{0.434} &
  \textbf{0.813} &
  \textbf{0.142} &
  \textbf{0.476} \\
 &
  \textit{Improvement} &
  \cellcolor[HTML]{EDFFED}\textit{0.50\%} &
  \cellcolor[HTML]{ECFFEC}\textit{0.53\%} &
  \cellcolor[HTML]{CFFFCF}\textit{1.34\%} &
  \cellcolor[HTML]{FAFFFA}\textit{0.16\%} &
  \cellcolor[HTML]{B9FFB9}\textit{1.93\%} &
  \cellcolor[HTML]{E3FFE3}\textit{0.77\%} \\ \bottomrule
\end{tabularx}%
}
\vspace{1em}
\caption{\textbf{Comparisons with different architecture pairs.} All experiments perform cross-task distillation from a classification teacher to a depth estimation student. The inverted projection is effective across various student model sizes and with different KD methods in this cross-task setting.}
\label{tab:rebuttal:enetb0-rn50-class2depth}
\end{table}

Table \ref{tab:rebuttal:enetb0-rn50-class2depth} shows results distilling from a classification teacher to a depth student using two student backbones of significantly-different sizes: an EfficientNet-B0 (5.3M params) and a ResNet-50 (25.6M params). These students are chosen to illustrate both a small and a large capacity gap between the student and teacher models.
Three different KD methods are used. Our inverted projector outperforms the traditional projector across all metrics for all three KD methods and both student backbone architectures in this cross-task setting, thus demonstrating the generality of our inverted projector for a variety of practical KD settings.
