# Supplementary material for: Learning to Project for Cross-Task Knowledge Distillation
Source: arXiv:2403.14494 source file (2024-11-27)
Supplement: Supplementary file 8 [file eigplots.tex]

\subsection{Training Dynamics of the Inverted Projector}
\label{sec:subsec:eigplots_section}

    \input{figures/SV_evolution_graphs} %
    
    By observing the singular value spectrum of the projector weights and how they evolve over the course of training, we are able to provide further insight into the role of our novel inverted projection for cross-task distillation, as compared to the traditional projection.
    Figure \ref{fig:eigplots} shows the singular value spectrum of the projector weights throughout the training process of a segmentation student with both similar and different teacher tasks, using either the traditional projection or our novel inverted projection.
    It can be seen that the traditional projection fails to disregard many of the less-dominant singular values, leading to a higher-rank projection in general.
    As discussed in section \ref{sec:subsec:why-does-proj-space-matter}, this is especially detrimental when there is a significant task gap, as it encourages the student to learn task-irrelevant features.
    When the student model is small, this can significantly degrade the target task performance. 
    However, when using our inverted projection, we observe a consistently lower rank across training for all tasks, compared to the traditional projection.
    This is because of the inverted projection's ability to suppress the task-irrelevant singular vectors from the teacher model: while the traditional projection remains consistently high-rank regardless of the dissimilarity of the student and teacher tasks, our inverted projection is able to adapt to discard the increasing quantity of undesirable task-specific knowledge encoded in the increasingly dissimilar teacher features.
