# Supplementary material for: Learning to Project for Cross-Task Knowledge Distillation
Source: arXiv:2403.14494 source file (2024-11-27)
Supplement: Supplementary file 9 [file eval-metrics.tex]

\subsection{Evaluation metrics}
\label{sec:app:metrics}
    \textbf{Monocular depth estimation.} We use the metrics defined in~\cite{eigen_depth_2014}: 
    \begin{itemize}
        \item Abs relative difference (Abs): $\frac{1}{T}\sum_{i=1}^{T} \frac{|d_i - d_i^*|}{d_i^*}$, 
        \item Squared relative difference (Sq): $\frac{1}{T}\sum_{i=1}^{T} \frac{||d_i - d_i^*||^2}{d_i^*}$, 
        \item RMSE (RMS): $\sqrt{\frac{1}{T}\sum_{i=0}^{T}\|d_i - d_i^*\|^2}$, 
        \item Log RMSE (RMSL): $\sqrt{\frac{1}{T}\sum_{i=0}^{T}\|log(d_i) - log(d_i^*)\|^2}$, 
        \item The threshold accuracy $\delta_n$: \(\%\) of \(d_i\) s.t. $max(\frac{d_i}{d_i^*}, \frac{d_i^*}{d_i}) = \delta < thr$, where $\delta_n$ denotes that $thr = 1.25^n$ (we use $n \in \{1, 2, 3\}$). $T$ denotes the total number of valid pixels in the ground truth depth map. $d_i$ and $d_i^*$ represent the predicted and ground-truth depth values at pixel $i$ respectively.
    \end{itemize}
