# Supplementary material for: Learning to Project for Cross-Task Knowledge Distillation
Source: arXiv:2403.14494 source file (2024-11-27)
Supplement: Supplementary file 10 [file full-MDE-results.tex]

\subsection{Full monocular depth estimation results}
\label{sec:app:full-results}
    
    Table \ref{tab:main_cross_task_distillation} shows only some metrics for monocular depth estimation (MDE) on NYUv2 \cite{silberman_indoor_2012} for the sake of brevity. We include here four additional tables showing the performance on all available metrics of a depth estimation student when distilled to from teachers trained for different tasks. Each table also includes metrics for the baseline, which is a student model trained without any distillation setup of any kind (i.e. only the task loss $\mathcal{L}_{task}$ is used). 
    Full details of the metrics used are in section \ref{sec:app:metrics}.
    See section \ref{sec:app:depth-student-models} for complete architectural details and section \ref{sec:app:loss-functions} for loss function details.

    \begin{table}
    \centering
    \scriptsize
    \begin{tabular}{ll|lllllll}
        \toprule
        \belowrulesepcolor{mygrey}
        \rowcolor{mygrey}
         &
           &
          \multicolumn{7}{c}{{\color{d2d} $\blacksquare$ } \textbf{Depth \textit{(Most similar)}} $\longrightarrow$ Depth} \\
        \rowcolor{mygrey} Method &
        Projection type &
          $\delta_1 \uparrow$ &
          $\delta_2 \uparrow$ &
          \multicolumn{1}{l|}{$\delta_3 \uparrow$} &
          Abs. Rel. $\downarrow$ &
          Sq. Rel. $\downarrow$ &
          RMS $\downarrow$ &
          RMSL $\downarrow$ \\ 
        \aboverulesepcolor{mygrey}
        \midrule
        \multicolumn{2}{c|}{\textit{No teacher (baseline)}} &
          \stackengine{2pt}{\textit{0.845}}{$_{\pm 0.007}$}{U}{c}{F}{T}{S} &
          \stackengine{2pt}{\textit{0.974}}{$_{\pm 0.001}$}{U}{c}{F}{T}{S} &
          \multicolumn{1}{l|}{\stackengine{2pt}{\textit{0.995}}{$_{\pm 0.000}$}{U}{c}{F}{T}{S}} &
          \stackengine{2pt}{\textit{0.127}}{$_{\pm 0.003}$}{U}{c}{F}{T}{S} &
          \stackengine{2pt}{\textit{0.078}}{$_{\pm 0.002}$}{U}{c}{F}{T}{S} &
          \stackengine{2pt}{\textit{0.440}}{$_{\pm 0.005}$}{U}{c}{F}{T}{S} &
          \stackengine{2pt}{\textit{0.160}}{$_{\pm 0.003}$}{U}{c}{F}{T}{S} \\
        \midrule
         &
          Traditional &
          \textbf{0.868} &
          \textbf{0.979} &
          \multicolumn{1}{l|}{\textbf{0.996}} &
          \textbf{0.117} &
          \textbf{0.069} &
          \textbf{0.406} &
          \textbf{0.148} \\
         &
          Inverted (Ours) &
          0.849 &
          0.976 &
          \multicolumn{1}{l|}{0.995} &
          0.124 &
          0.075 &
          0.432 &
          0.157 \\
        \multirow{-3}{*}{\begin{tabular}[c]{@{}l@{}}FitNets~\cite{romero_fitnets_2015} \\     \textit{\scriptsize ICLR 2015}\end{tabular}} &
          \textit{Improvement} &
          \cellcolor[HTML]{FFB0B0}\textit{-2.17\%} &
          \cellcolor[HTML]{FFF2F2}\textit{-0.34\%} &
          \multicolumn{1}{l|}{\cellcolor[HTML]{FFFEFE}\textit{-0.01\%}} &
          \cellcolor[HTML]{FF5858}\textit{-6.35\%} &
          \cellcolor[HTML]{FF5858}\textit{-9.66\%} &
          \cellcolor[HTML]{FF5858}\textit{-6.49\%} &
          \cellcolor[HTML]{FF5858}\textit{-5.92\%} \\ \midrule
         &
          Traditional &
          \textbf{0.856} &
          0.976 &
          \multicolumn{1}{l|}{\textbf{0.995}} &
          \textbf{0.122} &
          \textbf{0.073} &
          0.426 &
          \textbf{0.155} \\
         &
          Inverted (Ours) &
          \textbf{0.856} &
          \textbf{0.977} &
          \multicolumn{1}{l|}{\textbf{0.995}} &
          \textbf{0.122} &
          \textbf{0.073} &
          \textbf{0.425} &
          \textbf{0.155} \\
        \multirow{-3}{*}{\begin{tabular}[c]{@{}l@{}}AT~\cite{Zagoruyko2019PayingTransfer} \\  \textit{\scriptsize ICLR 2017}\end{tabular}} &
          \textit{Improvement} &
          \cellcolor[HTML]{FFFBFB}\textit{-0.11\%} &
          \cellcolor[HTML]{FDFFFD}\textit{0.06\%} &
          \multicolumn{1}{l|}{\cellcolor[HTML]{FFFFFF}\textit{0.01\%}} &
          \cellcolor[HTML]{FFFCFC}\textit{-0.08\%} &
          \cellcolor[HTML]{E2FFE2}\textit{0.82\%} &
          \cellcolor[HTML]{FFFFFF}\textit{0.02\%} &
          \cellcolor[HTML]{FFFFFF}\textit{0.00\%} \\ \midrule
         &
          Traditional &
          \textbf{0.854} &
          \textbf{0.978} &
          \multicolumn{1}{l|}{\textbf{0.996}} &
          \textbf{0.122} &
          \textbf{0.072} &
          0.429 &
          \textbf{0.155} \\
         &
          Inverted (Ours) &
          \textbf{0.854} &
          0.977 &
          \multicolumn{1}{l|}{\textbf{0.996}} &
          \textbf{0.122} &
          0.073 &
          \textbf{0.427} &
          \textbf{0.155} \\
        \multirow{-3}{*}{\begin{tabular}[c]{@{}l@{}}PKT~\cite{Passalis2018LearningTransfer} \\     \textit{\scriptsize ECCV 2018}\end{tabular}} &
          \textit{Improvement} &
          \cellcolor[HTML]{FEFFFE}\textit{0.04\%} &
          \cellcolor[HTML]{FFFBFB}\textit{-0.09\%} &
          \multicolumn{1}{l|}{\cellcolor[HTML]{FFFFFF}\textit{0.02\%}} &
          \cellcolor[HTML]{FFF9F9}\textit{-0.16\%} &
          \cellcolor[HTML]{FFCCCC}\textit{-1.38\%} &
          \cellcolor[HTML]{F0FFF0}\textit{0.42\%} &
          \cellcolor[HTML]{F8FFF8}\textit{0.19\%} \\ \midrule
         &
          Traditional &
          \textbf{0.861} &
          \textbf{0.978} &
          \multicolumn{1}{l|}{\textbf{0.996}} &
          \textbf{0.119} &
          \textbf{0.070} &
          \textbf{0.416} &
          \textbf{0.151} \\
         &
          Inverted (Ours) &
          0.849 &
          0.975 &
          \multicolumn{1}{l|}{\textbf{0.996}} &
          0.124 &
          0.076 &
          0.433 &
          0.157 \\
        \multirow{-3}{*}{\begin{tabular}[c]{@{}l@{}}Ensemble~\cite{Chen2022ImprovedEnsemble} \\    \textit{\scriptsize NeurIPS 2022}\end{tabular}} &
          \textit{Improvement} &
          \cellcolor[HTML]{FFC9C9}\textit{-1.46\%} &
          \cellcolor[HTML]{FFF4F4}\textit{-0.29\%} &
          \multicolumn{1}{l|}{\cellcolor[HTML]{FFFDFD}\textit{-0.05\%}} &
          \cellcolor[HTML]{FF5656}\textit{-4.64\%} &
          \cellcolor[HTML]{FF5858}\textit{-7.86\%} &
          \cellcolor[HTML]{FF6969}\textit{-4.11\%} &
          \cellcolor[HTML]{FF6464}\textit{-4.25\%} \\ 
          \bottomrule
    \end{tabular}
    \vspace{1em}
    \caption{\textbf{Depth teacher $\rightarrow$ Depth student (no task gap).} As expected, in same-task settings, our inverted projection produces a smaller improvement than the traditional projection. \textit{Improvement} is \% change using our inverted projection over using the traditional projection. See section \ref{sec:app:model_details} for model details. Baseline $\pm$ figures are variance from 3 runs.}
    \label{tab:supp:full-depth-table:depth-teacher}
\end{table}
\begin{table}
    \centering
    \scriptsize
    \begin{tabular}{ll|lllllll}
        \toprule
        \belowrulesepcolor{mygrey}
        \rowcolor{mygrey}
         &
           &
          \multicolumn{7}{c}{{\color{s2d} $\blacksquare$ } \textbf{Instance Segmentation} $\longrightarrow$ Depth} \\
        \rowcolor{mygrey} Method &
          Projection type &
          $\delta_1 \uparrow$ &
          $\delta_2 \uparrow$ &
          \multicolumn{1}{l|}{$\delta_3 \uparrow$} &
          Abs. Rel. $\downarrow$ &
          Sq. Rel. $\downarrow$ &
          RMS $\downarrow$ &
          RMSL $\downarrow$ \\  
        \aboverulesepcolor{mygrey}
        \midrule
        \multicolumn{2}{c|}{\textit{No teacher (baseline)}} &
          \stackengine{2pt}{\textit{0.845}}{$_{\pm 0.007}$}{U}{c}{F}{T}{S} &
          \stackengine{2pt}{\textit{0.974}}{$_{\pm 0.001}$}{U}{c}{F}{T}{S} &
          \multicolumn{1}{l|}{\stackengine{2pt}{\textit{0.995}}{$_{\pm 0.000}$}{U}{c}{F}{T}{S}} &
          \stackengine{2pt}{\textit{0.127}}{$_{\pm 0.003}$}{U}{c}{F}{T}{S} &
          \stackengine{2pt}{\textit{0.078}}{$_{\pm 0.002}$}{U}{c}{F}{T}{S} &
          \stackengine{2pt}{\textit{0.440}}{$_{\pm 0.005}$}{U}{c}{F}{T}{S} &
          \stackengine{2pt}{\textit{0.160}}{$_{\pm 0.003}$}{U}{c}{F}{T}{S} \\
         \midrule
         &
          Traditional &
          \textbf{0.855} &
          \textbf{0.977} &
          \multicolumn{1}{l|}{\textbf{0.996}} &
          \textbf{0.122} &
          \textbf{0.073} &
          \textbf{0.425} &
          \textbf{0.154} \\
         &
          Inverted (Ours) &
          0.851 &
          0.975 &
          \multicolumn{1}{l|}{0.995} &
          0.124 &
          0.075 &
          0.431 &
          0.157 \\
        \multirow{-3}{*}{\begin{tabular}[c]{@{}l@{}}FitNets~\cite{romero_fitnets_2015} \\     \textit{\scriptsize ICLR 2015}\end{tabular}} &
          \textit{Improvement} &
          \cellcolor[HTML]{FFF0F0}\textit{-0.41\%} &
          \cellcolor[HTML]{FFF5F5}\textit{-0.25\%} &
          \multicolumn{1}{l|}{\cellcolor[HTML]{FFFEFE}\textit{-0.02\%}} &
          \cellcolor[HTML]{FFBEBE}\textit{-1.78\%} &
          \cellcolor[HTML]{FFA3A3}\textit{-2.52\%} &
          \cellcolor[HTML]{FFCFCF}\textit{-1.31\%} &
          \cellcolor[HTML]{FFC1C1}\textit{-1.68\%} \\ \midrule
         &
          Traditional &
          0.852 &
          0.976 &
          \multicolumn{1}{l|}{\textbf{0.995}} &
          0.123 &
          0.075 &
          0.431 &
          0.156 \\
         &
          Inverted (Ours) &
          \textbf{0.855} &
          \textbf{0.978} &
          \multicolumn{1}{l|}{\textbf{0.995}} &
          \textbf{0.121} &
          \textbf{0.073} &
          \textbf{0.429} &
          \textbf{0.155} \\
        \multirow{-3}{*}{\begin{tabular}[c]{@{}l@{}}AT~\cite{Zagoruyko2019PayingTransfer} \\  \textit{\scriptsize ICLR 2017}\end{tabular}} &
          \textit{Improvement} &
          \cellcolor[HTML]{F0FFF0}\textit{0.42\%} &
          \cellcolor[HTML]{FAFFFA}\textit{0.16\%} &
          \multicolumn{1}{l|}{\cellcolor[HTML]{FFFFFF}\textit{0.00\%}} &
          \cellcolor[HTML]{CDFFCD}\textit{1.38\%} &
          \cellcolor[HTML]{C0FFC0}\textit{1.74\%} &
          \cellcolor[HTML]{ECFFEC}\textit{0.53\%} &
          \cellcolor[HTML]{E3FFE3}\textit{0.77\%} \\ \midrule
         &
          Traditional &
          \textbf{0.857} &
          \textbf{0.976} &
          \multicolumn{1}{l|}{\textbf{0.995}} &
          \textbf{0.123} &
          \textbf{0.075} &
          \textbf{0.427} &
          \textbf{0.155} \\
         &
          Inverted (Ours) &
          0.854 &
          \textbf{0.976} &
          \multicolumn{1}{l|}{\textbf{0.995}} &
          \textbf{0.123} &
          \textbf{0.075} &
          0.429 &
          0.156 \\
        \multirow{-3}{*}{\begin{tabular}[c]{@{}l@{}}PKT~\cite{Passalis2018LearningTransfer} \\     \textit{\scriptsize ECCV 2018}\end{tabular}} &
          \textit{Improvement} &
          \cellcolor[HTML]{FFF2F2}\textit{-0.34\%} &
          \cellcolor[HTML]{FEFFFE}\textit{0.04\%} &
          \multicolumn{1}{l|}{\cellcolor[HTML]{FFFFFF}\textit{0.01\%}} &
          \cellcolor[HTML]{FFFCFC}\textit{-0.08\%} &
          \cellcolor[HTML]{FFFAFA}\textit{-0.13\%} &
          \cellcolor[HTML]{FFEEEE}\textit{-0.44\%} &
          \cellcolor[HTML]{FFECEC}\textit{-0.52\%} \\ \midrule
         &
          Traditional &
          \textbf{0.856} &
          \textbf{0.977} &
          \multicolumn{1}{l|}{\textbf{0.996}} &
          \textbf{0.122} &
          \textbf{0.072} &
          \textbf{0.425} &
          \textbf{0.154} \\
         &
          Inverted (Ours) &
          0.848 &
          0.975 &
          \multicolumn{1}{l|}{0.995} &
          0.124 &
          0.076 &
          0.435 &
          0.157 \\
        \multirow{-3}{*}{\begin{tabular}[c]{@{}l@{}}Ensemble~\cite{Chen2022ImprovedEnsemble} \\     \textit{\scriptsize NeurIPS 2022}\end{tabular}} &
          \textit{Improvement} &
          \cellcolor[HTML]{FFDCDC}\textit{-0.95\%} &
          \cellcolor[HTML]{FFF9F9}\textit{-0.16\%} &
          \multicolumn{1}{l|}{\cellcolor[HTML]{FFFDFD}\textit{-0.05\%}} &
          \cellcolor[HTML]{FFC3C3}\textit{-1.64\%} &
          \cellcolor[HTML]{FF5353}\textit{-4.70\%} &
          \cellcolor[HTML]{FFB0B0}\textit{-2.16\%} &
          \cellcolor[HTML]{FFBABA}\textit{-1.88\%} \\
          \bottomrule
    \end{tabular}
    \vspace{1em}
    \caption{\textbf{Instance segmentation teacher $\rightarrow$ Depth student (small task gap).} The two tasks are different, but are similar enough that the traditional projection produces greater improvements than our inverted projection does with most methods. \textit{Improvement} is \% change using our inverted projection over using the traditional projection. See section \ref{sec:app:model_details} for model details. Baseline $\pm$ figures are variance from 3 runs.}
    \label{tab:supp:full-depth-table:insseg-teacher}
\end{table}
\begin{table}
    \centering
    \scriptsize
    \begin{tabular}{ll|lllllll}
        \toprule
        \belowrulesepcolor{mygrey}
        \rowcolor{mygrey}
         &
           &
          \multicolumn{7}{c}{{\color{c2d} $\blacksquare$ } \textbf{Classification} $\longrightarrow$ Depth} \\
        \rowcolor{mygrey} Method &
          Projection type &
          $\delta_1 \uparrow$ &
          $\delta_2 \uparrow$ &
          \multicolumn{1}{l|}{$\delta_3 \uparrow$} &
          Abs. Rel. $\downarrow$ &
          Sq. Rel. $\downarrow$ &
          RMS $\downarrow$ &
          RMSL $\downarrow$ \\ 
        \aboverulesepcolor{mygrey}
        \midrule
        \multicolumn{2}{c|}{\textit{No teacher (baseline)}} &
          \stackengine{2pt}{\textit{0.845}}{$_{\pm 0.007}$}{U}{c}{F}{T}{S} &
          \stackengine{2pt}{\textit{0.974}}{$_{\pm 0.001}$}{U}{c}{F}{T}{S} &
          \multicolumn{1}{l|}{\stackengine{2pt}{\textit{0.995}}{$_{\pm 0.000}$}{U}{c}{F}{T}{S}} &
          \stackengine{2pt}{\textit{0.127}}{$_{\pm 0.003}$}{U}{c}{F}{T}{S} &
          \stackengine{2pt}{\textit{0.078}}{$_{\pm 0.002}$}{U}{c}{F}{T}{S} &
          \stackengine{2pt}{\textit{0.440}}{$_{\pm 0.005}$}{U}{c}{F}{T}{S} &
          \stackengine{2pt}{\textit{0.160}}{$_{\pm 0.003}$}{U}{c}{F}{T}{S} \\
         \midrule
         &
          Traditional &
          0.845 &
          \textbf{0.976} &
          \multicolumn{1}{l|}{\textbf{0.996}} &
          0.125 &
          0.076 &
          0.439 &
          0.158 \\
         &
          Inverted (Ours) &
          \textbf{0.850} &
          0.975 &
          \multicolumn{1}{l|}{\textbf{0.995}} &
          \textbf{0.124} &
          \textbf{0.075} &
          \textbf{0.434} &
          \textbf{0.157} \\
        \multirow{-3}{*}{\begin{tabular}[c]{@{}l@{}}FitNets~\cite{romero_fitnets_2015} \\     \textit{\scriptsize ICLR 2015}\end{tabular}} &
          \textit{Improvement} &
          \cellcolor[HTML]{EDFFED}\textit{0.50\%} &
          \cellcolor[HTML]{FFFCFC}\textit{-0.06\%} &
          \multicolumn{1}{l|}{\cellcolor[HTML]{FFFDFD}\textit{-0.03\%}} &
          \cellcolor[HTML]{ECFFEC}\textit{0.53\%} &
          \cellcolor[HTML]{EFFFEF}\textit{0.44\%} &
          \cellcolor[HTML]{CFFFCF}\textit{1.34\%} &
          \cellcolor[HTML]{E2FFE2}\textit{0.80\%} \\ \midrule
         &
          Traditional &
          0.850 &
          \textbf{0.976} &
          \multicolumn{1}{l|}{\textbf{0.995}} &
          0.125 &
          0.076 &
          0.433 &
          0.157 \\
         &
          Inverted (Ours) &
          \textbf{0.853} &
          \textbf{0.976} &
          \multicolumn{1}{l|}{\textbf{0.995}} &
          \textbf{0.123} &
          \textbf{0.074} &
          \textbf{0.430} &
          \textbf{0.156} \\
        \multirow{-3}{*}{\begin{tabular}[c]{@{}l@{}}AT~\cite{Zagoruyko2019PayingTransfer} \\ \textit{\scriptsize ICLR 2017}\end{tabular}} &
          \textit{Improvement} &
          \cellcolor[HTML]{F3FFF3}\textit{0.35\%} &
          \cellcolor[HTML]{FDFFFD}\textit{0.08\%} &
          \multicolumn{1}{l|}{\cellcolor[HTML]{FFFFFF}\textit{0.02\%}} &
          \cellcolor[HTML]{C5FFC5}\textit{1.61\%} &
          \cellcolor[HTML]{91FF91}\textit{3.03\%} &
          \cellcolor[HTML]{E3FFE3}\textit{0.79\%} &
          \cellcolor[HTML]{E1FFE1}\textit{0.83\%} \\ \midrule
         &
          Traditional &
          0.851 &
          0.975 &
          \multicolumn{1}{l|}{\textbf{0.996}} &
          0.124 &
          0.076 &
          0.432 &
          0.157 \\
         &
          Inverted (Ours) &
          \textbf{0.853} &
          \textbf{0.976} &
          \multicolumn{1}{l|}{0.995} &
          \textbf{0.123} &
          \textbf{0.074} &
          \textbf{0.431} &
          \textbf{0.156} \\
        \multirow{-3}{*}{\begin{tabular}[c]{@{}l@{}}PKT~\cite{Passalis2018LearningTransfer} \\     \textit{\scriptsize ECCV 2018}\end{tabular}} &
          \textit{Improvement} &
          \cellcolor[HTML]{F7FFF7}\textit{0.25\%} &
          \cellcolor[HTML]{FEFFFE}\textit{0.05\%} &
          \multicolumn{1}{l|}{\cellcolor[HTML]{FFFDFD}\textit{-0.03\%}} &
          \cellcolor[HTML]{D1FFD1}\textit{1.29\%} &
          \cellcolor[HTML]{A5FFA5}\textit{2.50\%} &
          \cellcolor[HTML]{F5FFF5}\textit{0.30\%} &
          \cellcolor[HTML]{E8FFE8}\textit{0.64\%} \\ \midrule
         &
          Traditional &
          \textbf{0.852} &
          \textbf{0.976} &
          \multicolumn{1}{l|}{\textbf{0.995}} &
          \textbf{0.124} &
          \textbf{0.075} &
          \textbf{0.431} &
          \textbf{0.156} \\
         &
          Inverted (Ours) &
          0.847 &
          0.975 &
          \multicolumn{1}{l|}{\textbf{0.995}} &
          0.125 &
          0.076 &
          0.437 &
          0.158 \\
        \multirow{-3}{*}{\begin{tabular}[c]{@{}l@{}}Ensemble~\cite{Chen2022ImprovedEnsemble} \\     \textit{\scriptsize NeurIPS 2022}\end{tabular}} &
          \textit{Improvement} &
          \cellcolor[HTML]{FFE7E7}\textit{-0.63\%} &
          \cellcolor[HTML]{FFFAFA}\textit{-0.12\%} &
          \multicolumn{1}{l|}{\cellcolor[HTML]{FFFFFF}\textit{0.02\%}} &
          \cellcolor[HTML]{FFDEDE}\textit{-0.89\%} &
          \cellcolor[HTML]{FFC4C4}\textit{-1.61\%} &
          \cellcolor[HTML]{FFCFCF}\textit{-1.30\%} &
          \cellcolor[HTML]{FFD7D7}\textit{-1.09\%} \\
          \bottomrule
    \end{tabular}
    \vspace{1em}
    \caption{\textbf{Classification teacher $\rightarrow$ Depth student (larger task gap).} The two tasks are different enough that the setting becomes more ``cross-task" than ``same-task", and our inverted projection begins to outperform the traditional student model in terms of improvement over the baseline. \textit{Improvement} is \% change using our inverted projection over using the traditional projection. See section \ref{sec:app:model_details} for model details. Baseline $\pm$ figures are variance from 3 runs.}
    \label{tab:supp:full-depth-table:class-teacher}
\end{table}
\begin{table}
    \centering
    \scriptsize
    \begin{tabular}{ll|lllllll}
        \toprule
        \belowrulesepcolor{mygrey}
        \rowcolor{mygrey}
         &
           &
          \multicolumn{7}{c}{{\color{r2d} $\blacksquare$ } \textbf{Random \textit{(Least similar)}} $\longrightarrow$ Depth} \\
        \rowcolor{mygrey} Method &
          Projection type &
          $\delta_1 \uparrow$ &
          $\delta_2 \uparrow$ &
          \multicolumn{1}{l|}{$\delta_3 \uparrow$} &
          Abs. Rel. $\downarrow$ &
          Sq. Rel. $\downarrow$ &
          RMS $\downarrow$ &
          RMSL $\downarrow$ \\ 
        \aboverulesepcolor{mygrey}
        \midrule
        \multicolumn{2}{c|}{\textit{No teacher (baseline)}} &
          \stackengine{2pt}{\textit{0.845}}{$_{\pm 0.007}$}{U}{c}{F}{T}{S} &
          \stackengine{2pt}{\textit{0.974}}{$_{\pm 0.001}$}{U}{c}{F}{T}{S} &
          \multicolumn{1}{l|}{\stackengine{2pt}{\textit{0.995}}{$_{\pm 0.000}$}{U}{c}{F}{T}{S}} &
          \stackengine{2pt}{\textit{0.127}}{$_{\pm 0.003}$}{U}{c}{F}{T}{S} &
          \stackengine{2pt}{\textit{0.078}}{$_{\pm 0.002}$}{U}{c}{F}{T}{S} &
          \stackengine{2pt}{\textit{0.440}}{$_{\pm 0.005}$}{U}{c}{F}{T}{S} &
          \stackengine{2pt}{\textit{0.160}}{$_{\pm 0.003}$}{U}{c}{F}{T}{S} \\
         \midrule
         &
          Traditional &
          0.828 &
          0.970 &
          \multicolumn{1}{l|}{\textbf{0.995}} &
          0.134 &
          0.084 &
          0.455 &
          0.167 \\
         &
          Inverted (Ours) &
          \textbf{0.851} &
          \textbf{0.976} &
          \multicolumn{1}{l|}{\textbf{0.995}} &
          \textbf{0.124} &
          \textbf{0.075} &
          \textbf{0.431} &
          \textbf{0.156} \\
        \multirow{-3}{*}{\begin{tabular}[c]{@{}l@{}}FitNets~\cite{romero_fitnets_2015} \\     \textit{\scriptsize ICLR 2015}\end{tabular}} &
          \textit{Improvement} &
          \cellcolor[HTML]{97FF97}\textit{2.86\%} &
          \cellcolor[HTML]{EAFFEA}\textit{0.58\%} &
          \multicolumn{1}{l|}{\cellcolor[HTML]{FDFFFD}\textit{0.08\%}} &
          \cellcolor[HTML]{00FF00}\textit{7.47\%} &
          \cellcolor[HTML]{00FF00}\textit{11.15\%} &
          \cellcolor[HTML]{42FF42}\textit{5.20\%} &
          \cellcolor[HTML]{18FF18}\textit{6.36\%} \\ \midrule
         &
          Traditional &
          \textbf{0.857} &
          \textbf{0.977} &
          \multicolumn{1}{l|}{\textbf{0.996}} &
          \textbf{0.121} &
          \textbf{0.073} &
          \textbf{0.428} &
          \textbf{0.154} \\
         &
          Inverted (Ours) &
          \textbf{0.857} &
          0.976 &
          \multicolumn{1}{l|}{0.995} &
          0.122 &
          0.074 &
          \textbf{0.428} &
          0.155 \\
        \multirow{-3}{*}{\begin{tabular}[c]{@{}l@{}}AT~\cite{Zagoruyko2019PayingTransfer} \\ \textit{\scriptsize ICLR 2017}\end{tabular}} &
          \textit{Improvement} &
          \cellcolor[HTML]{FEFFFE}\textit{0.05\%} &
          \cellcolor[HTML]{FFFDFD}\textit{-0.04\%} &
          \multicolumn{1}{l|}{\cellcolor[HTML]{FFFDFD}\textit{-0.03\%}} &
          \cellcolor[HTML]{FFE0E0}\textit{-0.83\%} &
          \cellcolor[HTML]{FFCCCC}\textit{-1.37\%} &
          \cellcolor[HTML]{FCFFFC}\textit{0.09\%} &
          \cellcolor[HTML]{FFF0F0}\textit{-0.39\%} \\ \midrule
         &
          Traditional &
          0.856 &
          0.975 &
          \multicolumn{1}{l|}{\textbf{0.995}} &
          0.123 &
          0.075 &
          0.429 &
          \textbf{0.155} \\
         &
          Inverted (Ours) &
          \textbf{0.858} &
          \textbf{0.976} &
          \multicolumn{1}{l|}{\textbf{0.995}} &
          \textbf{0.122} &
          \textbf{0.073} &
          \textbf{0.426} &
          \textbf{0.155} \\
        \multirow{-3}{*}{\begin{tabular}[c]{@{}l@{}}PKT~\cite{Passalis2018LearningTransfer} \\     \textit{\scriptsize ECCV 2018}\end{tabular}} &
          \textit{Improvement} &
          \cellcolor[HTML]{F5FFF5}\textit{0.29\%} &
          \cellcolor[HTML]{FCFFFC}\textit{0.10\%} &
          \multicolumn{1}{l|}{\cellcolor[HTML]{FFFFFF}\textit{0.00\%}} &
          \cellcolor[HTML]{D3FFD3}\textit{1.22\%} &
          \cellcolor[HTML]{99FF99}\textit{2.80\%} &
          \cellcolor[HTML]{E1FFE1}\textit{0.84\%} &
          \cellcolor[HTML]{EAFFEA}\textit{0.58\%} \\ \midrule
         &
          Traditional &
          0.835 &
          0.973 &
          \multicolumn{1}{l|}{0.995} &
          0.128 &
          0.079 &
          0.446 &
          0.162 \\
         &
          Inverted (Ours) &
          \textbf{0.849} &
          \textbf{0.976} &
          \multicolumn{1}{l|}{\textbf{0.996}} &
          \textbf{0.124} &
          \textbf{0.075} &
          \textbf{0.432} &
          \textbf{0.157} \\
        \multirow{-3}{*}{\begin{tabular}[c]{@{}l@{}}Ensemble~\cite{Chen2022ImprovedEnsemble} \\     \textit{\scriptsize NeurIPS 2022}\end{tabular}} &
          \textit{Improvement} &
          \cellcolor[HTML]{C0FFC0}\textit{1.74\%} &
          \cellcolor[HTML]{F6FFF6}\textit{0.26\%} &
          \multicolumn{1}{l|}{\cellcolor[HTML]{FDFFFD}\textit{0.06\%}} &
          \cellcolor[HTML]{9BFF9B}\textit{2.75\%} &
          \cellcolor[HTML]{4BFF4B}\textit{4.96\%} &
          \cellcolor[HTML]{91FF91}\textit{3.03\%} &
          \cellcolor[HTML]{84FF84}\textit{3.39\%} \\
        \bottomrule
    \end{tabular}
    \vspace{1em}
    \caption{\textbf{Randomly-initialised teacher $\rightarrow$ Depth student (largest task gap).} Our inverted projection produces significant improvement. \textit{Improvement} is \% change using our inverted projection over using the traditional projection. See section \ref{sec:app:model_details} for model details. Baseline $\pm$ figures are variance from 3 runs.}
    \label{tab:supp:full-depth-table:random-teacher}
\end{table}
    
    Each table shows a single teacher/student task pair, and compares four different knowledge distillation methods when using both the traditional projection and our inverted projection, as well as including a percentage \textit{Improvement} showing the difference in performance when using our inverted projection compared to the traditional projection.

    % \newpage
    Table \ref{tab:supp:full-depth-table:depth-teacher} shows results using a depth estimation teacher. As the teacher and student tasks are identical and the task-specific features in the teacher are desired for the student model, the traditional projection produces a greater performance improvement than our inverted projection.
    
    Table \ref{tab:supp:full-depth-table:insseg-teacher} shows results using an instance segmentation teacher. Instance segmentation produces both semantic labels and instance labels, and the semantic masks and labels are known to be useful for depth estimation (see section \ref{sec:related_work}), so while the teacher and student tasks are different, they are similar to one another. Therefore, we see that the traditional projection still outperforms our inverted projection in most cases, as expected.
    
    Table \ref{tab:supp:full-depth-table:class-teacher} shows results with a classification teacher. This is a cross-task setup: classification is relatively unrelated to monocular depth estimation. As a result, it can be seen that our inverted projection outperforms the traditional projection.
    
    Table \ref{tab:supp:full-depth-table:random-teacher} shows results with a randomly-initialised and frozen teacher model. The randomly-initialised teacher does not contain any task-specific knowledge whatsoever, and therefore the task-gap between the teacher and the student model is maximised. As this is the most cross-task setting, our inverted projection performs the best in comparison to the traditional projection, as it is only our inverted projection that is able to successfully discard the confounding features present in the randomly-initialised teacher.

    \input{figures/qualitative_figures}    

    We also provide qualitative examples using same-task, similar-task, and randomly-initialised teachers on a different depth estimation student, shown in figure \ref{fig:qualitative-different-teachers}. In all cases, we are able to obtain qualitatively good performance.
