# Supplementary material for: Learning to Project for Cross-Task Knowledge Distillation
Source: arXiv:2403.14494 source file (2024-11-27)
Supplement: Supplementary file 11 [file linear-mapping.tex]

\subsection{Linear mapping between task spaces}
\label{sec:subsec:linear-mapping-between}

\begin{figure}
    \centering
    \subfigure[Input Image]{\hspace{.3\textwidth}}
    \subfigure[Predicted Depth]{\hspace{.3\textwidth}}
    
    \subfigure{\includegraphics[width=0.3\textwidth]{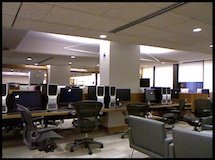}}
    \subfigure{\includegraphics[width=0.3\textwidth]{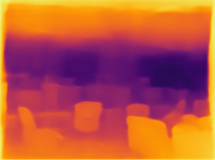}}
    
    \subfigure{\includegraphics[width=0.3\textwidth]{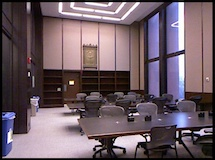}}
    \subfigure{\includegraphics[width=0.3\textwidth]{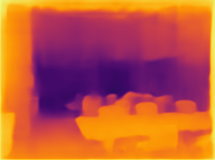}}
    \vspace{1em}
    \caption{\textbf{Qualitative results using a frozen segmentation encoder and frozen depth decoder.} With only a learned linear projection, features from the semantic segmentation task can be made immediately useful for depth.}
    \label{fig:qualitative_toy_experiment}
\end{figure}

In performing cross-task distillation, we assume there is an overlap in information in the representation spaces across different tasks, following both the work in the literature and intuition (see section \ref{sec:related_work}). 
\cite{merullo_linearly_2022} demonstrated the existence of a learnable linear mapping between text and image features. Concurrently, research has shown that linear projections are very effective for knowledge distillation\cite{Chen2022ImprovedEnsemble, miles2024understanding}. However, a natural unification of these two settings has not been explored.

We experimentally verify the validity of this assumption with a simple toy scenario, in which a frozen encoder pretrained on instance segmentation is connected via a learnable linear projection to a frozen decoder pretrained for depth estimation. Example qualitative results in figure \ref{fig:qualitative_toy_experiment} show that the linearly projected cross-task features can be successfully utilized to generate a coherent output, despite both models being frozen. In fact, by only training the linear projector between these two frozen models, we can attain $0.504$ RMSE on NYUv2. This result indicates that a significant portion of the information contained in the instance segmentation features are closely related to the depth estimation task. We conduct additional experiments projecting between various other task representation spaces.
These results indicate that cross-task distillation using linear projection is a promising approach for leveraging shared information between specific pairs of tasks, and further motivate our work.
