# Supplementary material for: Learning to Project for Cross-Task Knowledge Distillation
Source: arXiv:2403.14494 source file (2024-11-27)
Supplement: Supplementary file 12 [file model-details.tex]

\subsection{Model details}
\label{sec:app:model_details}
    This section details the different student and teacher architectures used for our experiments.

    \subsubsection{Depth estimation}
    \label{sec:app:depth_est_models}
        \paragraph{Teacher models:}
            The teacher models used for depth estimation are:
            \begin{itemize}
                \item 
                    \textbf{Depth teacher}: SwinV2-B \cite{liu_swin_2022} pretrained on NYUv2 as part of the All In Tokens \cite{ning_all_2023} framework.
                    \footnote{\url{https://msravcghub.blob.core.windows.net/ait-release/checkpoint/ait\_depth\_swinv2b\_ar.pth}},
                    available from the official AiT repository\footnote{\url{https://github.com/SwinTransformer/AiT}}.
                \item 
                    \textbf{Instance segmentation teacher}: SwinV2-B pretrained on COCO \cite{Lin2014MicrosoftContext} as part of the All In Tokens framework.
                \item 
                    \textbf{Classification teacher}: ViT-B-16 pretrained on ImageNet-1K, available from the torchvision model hub\footnote{\label{footnote:torchvision-models}\url{https://pytorch.org/vision/stable/models.html}}.
            \end{itemize}

        \paragraph{Student Models:}
        \label{sec:app:depth-student-models}
            The depth estimation students used have one of three backbones:
            \begin{itemize}
                \item MobilenetV2 \cite{Fox2018MobileNetV2:Bottlenecks}: In our experiments, we use a width multiplier of 0.5.
                \item EfficientNet-B0 \cite{tan_efficientnet_2019}.
                \item ResNet-50 \cite{He2015ResNetRecognition}.
            \end{itemize}
            The decoders used are (names in \texttt{this font}):
            \begin{itemize}
                \item \texttt{Decoder}:
                    Conv1x1, then 6 blocks of (LeakyReLU + Conv3x3 + LeakyReLU + Conv3x3). At the input to each of the 6 blocks, an incoming skip connection from the encoder is bilinearly upsampled to match the feature resolution, then concatenated to the features.
                \item \texttt{Decoder\_dl2}:
                    The same as \texttt{Decoder}, except the second Conv3x3 in each block is replaced with a depthwise convolution to reduce parameters.
                \item \texttt{ULightDecoder\_skip\_4b}:
                    Conv1x1, then 4 blocks of (LeakyReLU + Conv3x3). As in the other decoders, each block receives features from an incoming skip connection, which are upsampled to match the feature resolution and then concatenated.
            \end{itemize}

    \subsubsection{Semantic segmentation}
        \paragraph{Teacher models:}
            The teacher models used for semantic segmentation are:
            \begin{itemize}
                \item Segmentation teacher:
                    A DeepLab-V3 \cite{chen_rethinking_2017} with a ResNet-50 backbone, pretrained on a subset of MSCOCO that uses only the 20 categories present in the Pascal VOC dataset. Model and checkpoint loaded from torchvision model hub\footnotemark[\getrefnumber{footnote:torchvision-models}].
                \item Classification teacher: 
                    ResNet-50 \cite{He2015ResNetRecognition} pretrained on ImageNet-1K. Model and checkpoint loaded from torchvision model hub\footnotemark[\getrefnumber{footnote:torchvision-models}].
            \end{itemize}
        \paragraph{Student model:}
            The student model used for semantic segmentation was a DeepLabV3 \cite{chen_deeplab:_2017} with a ResNet50 backbone that is pretrained on ImageNet-1K. The pretrained weights were sourced from the torchvision model hub\footnotemark[\getrefnumber{footnote:torchvision-models}].

    \subsubsection{Satellite-to-map and Colorization}
        We use the same teacher models described in section \ref{sec:app:depth_est_models}. For the student models on the satellite-to-map experiments, we use a CycleGAN, while for the colorization experiments we use a Pix2Pix model. This Pix2Pix model follows a standard UNet-like architecture with batch norm layers.
