# Supplementary material for: Learning to Project for Cross-Task Knowledge Distillation
Source: arXiv:2403.14494 source file (2024-11-27)
Supplement: Supplementary file 13 [file task-losses.tex]

\subsection{Task losses}
\label{sec:app:loss-functions}
    In addition to the projection loss $\mathcal{L}_{distill}$, each student is trained with a task-specific loss $\mathcal{L}_{task}$ to supervise its output. The task and projection loss components are weighted equally, as in equation \ref{eq:total_loss}.

    The depth task loss function used is a variant of the Scale-Invariant Log-Loss (SILog), first proposed by \cite{eigen_depth_2014} and modified by \cite{bhat_adabins_2020}:
        \begin{equation}
        \label{eq:depth-loss}
        \mathcal{L}_{SILog} = 10 \sqrt{\frac{1}{K}\displaystyle\sum^K_{i = 1} g_{i}^2 + \frac{0.15}{K^2}\left(\displaystyle\sum^K_{i = 1} g_{i}\right)^2}
    \end{equation}
    where ground-truth and predicted depth values for pixel $i$ are given as $d^*_i$ and $d_i$ respectively, $g_{i} = log(d_{i}) - log(d^*_{i})$ and $K$ is the total number of pixels with valid depth values.
    Semantic segmentation students are trained with a pixelwise cross-entropy loss.
    For the colourization task we use the vanilla GAN loss\cite{Goodfellow2014GenerativeNetworks} in addition to an L1 loss with a weighting of $100.0$. For the satellite-to-map translation we use the cyclic consistency loss described in the original CycleGAN paper~\cite{Zhu2017UnpairedNetworks}.
