# Supplementary material for: Learning to Project for Cross-Task Knowledge Distillation
Source: arXiv:2403.14494 source file (2024-11-27)
Supplement: Supplementary file 14 [file teacher_free_results.tex]

\subsection{Teacher-Free Distillation: Results}

\begin{table}
    \centering
    \footnotesize
    \begin{tabular}{lccc}
        \toprule
        \belowrulesepcolor{mygrey}
        \rowcolor{mygrey} Method & RMS $\downarrow$ & Abs $\downarrow$ & $\delta_1$ $\uparrow$ \\
        \aboverulesepcolor{mygrey}
        \midrule
        \textit{(Baseline) AiT (SwinV2-B) \cite{ning_all_2023}} & \textit{0.365}            & \textit{0.105}            & \textit{0.907}                 \\
        \midrule
         $\mathcal{L}_{spectral}$ $(r = 1)$              & 0.352            & 0.105            & 0.902                 \\
         $\mathcal{L}_{spectral}$ $(r = 2)$              & \textbf{0.340}   & \textbf{0.096}   & \textbf{0.914}        \\
         $\mathcal{L}_{spectral}$ $(r = 4)$              & 0.349            & 0.099            & 0.911                 \\
         $\mathcal{L}_{spectral}$ $(r = 8)$              & 0.344            & \textbf{0.096}   & 0.910                 \\
         $\mathcal{L}_{spectral}$ $(r = 16)$             & 0.348            & 0.098            & 0.912                 \\
         $\mathcal{L}_{spectral}$ $(r = 32)$             & 0.347            & 0.100            & 0.909                 \\
        \bottomrule
    \end{tabular}
    \vspace{1em}
    \caption{\textbf{Teacher-free distillation} using our spectral regularisation loss on the NYUv2 dataset using AiT \cite{ning_all_2023} on a SwinV2-b base. The regularisation loss is generally robust to different values of $r$, with $r = 2$ being optimal.
    }
    \label{tab:manual-reg-ait}
\end{table}

Table \ref{tab:manual-reg-ait} shows the performance of the teacher-free distillation strategy detailed in section \ref{sec:subsec:experiments-ablation-study-teacher-free-backbones} using different ranks, when applied to a depth estimation setup. A higher value of $r$ uses more of the available principal components to reconstruct the features. The optimal value is found to be when $r=2$.
