# Supplementary material for: Learning to Project for Cross-Task Knowledge Distillation
Source: arXiv:2403.14494 source file (2024-11-27)
Supplement: Supplementary file 15 [file training-details.tex]

% \subsection{Training details}
% \label{sec:app:training-details}
\subsection{Hyperparameters}
\label{sec:app:training-details}
\vspace{0.5em}\textbf{Monocular depth estimation.} Depth estimation students were trained for 25 epochs using the AdamW optimizer with a learning rate of 2e-4 and weight decay of 0.05. The OneCycle learning rate scheduler was used \cite{smith_super-convergence_2018} with the maximum learning rate set to 2e-4. The batch size was set to 16.

\vspace{0.5em}\noindent\textbf{Semantic segmentation.} Semantic segmentation students were trained for 80 epochs using the AdamW optimizer with a learning rate of 5e-3 and weight decay of 1e-2. The OneCycle learning rate scheduler was used, with the maximum learning rate set to 5e-3. The batch size was set to 20.

\vspace{0.5em}\noindent\textbf{Image-to-image translation (satellite-to-map, colorization).} Each model for both of these tasks are trained for 200 epochs using the AdamW optimizer with a learning rate of 2e-4. We keep the initial learning rate for the first 100 epochs and then linearly decay the rate to zero over the next 100 epochs with a batch size of 8.
