# Supplementary material for: Learning to Project for Cross-Task Knowledge Distillation
Source: arXiv:2403.14494 source file (2024-11-27)
Supplement: Supplementary file 16 [file full_depth_table.tex]

\begin{table}
    \centering
    \scriptsize
    \begin{tabular}{ll|lllllll}
        \toprule
        \belowrulesepcolor{mygrey}
        \rowcolor{mygrey}
         &
           &
          \multicolumn{7}{c}{{\color{d2d} $\blacksquare$ } \textbf{Depth \textit{(Most similar)}} $\longrightarrow$ Depth} \\
        \rowcolor{mygrey} Method &
        Projection type &
          $\delta_1 \uparrow$ &
          $\delta_2 \uparrow$ &
          \multicolumn{1}{l|}{$\delta_3 \uparrow$} &
          Abs. Rel. $\downarrow$ &
          Sq. Rel. $\downarrow$ &
          RMS $\downarrow$ &
          RMSL $\downarrow$ \\ 
        \aboverulesepcolor{mygrey}
        \midrule
        \multicolumn{2}{c|}{\textit{No teacher (baseline)}} &
          \stackengine{2pt}{\textit{0.845}}{$_{\pm 0.007}$}{U}{c}{F}{T}{S} &
          \stackengine{2pt}{\textit{0.974}}{$_{\pm 0.001}$}{U}{c}{F}{T}{S} &
          \multicolumn{1}{l|}{\stackengine{2pt}{\textit{0.995}}{$_{\pm 0.000}$}{U}{c}{F}{T}{S}} &
          \stackengine{2pt}{\textit{0.127}}{$_{\pm 0.003}$}{U}{c}{F}{T}{S} &
          \stackengine{2pt}{\textit{0.078}}{$_{\pm 0.002}$}{U}{c}{F}{T}{S} &
          \stackengine{2pt}{\textit{0.440}}{$_{\pm 0.005}$}{U}{c}{F}{T}{S} &
          \stackengine{2pt}{\textit{0.160}}{$_{\pm 0.003}$}{U}{c}{F}{T}{S} \\
        \midrule
         &
          Traditional &
          \textbf{0.868} &
          \textbf{0.979} &
          \multicolumn{1}{l|}{\textbf{0.996}} &
          \textbf{0.117} &
          \textbf{0.069} &
          \textbf{0.406} &
          \textbf{0.148} \\
         &
          Inverted (Ours) &
          0.849 &
          0.976 &
          \multicolumn{1}{l|}{0.995} &
          0.124 &
          0.075 &
          0.432 &
          0.157 \\
        \multirow{-3}{*}{\begin{tabular}[c]{@{}l@{}}FitNets~\cite{romero_fitnets_2015} \\     \textit{\scriptsize ICLR 2015}\end{tabular}} &
          \textit{Improvement} &
          \cellcolor[HTML]{FFB0B0}\textit{-2.17\%} &
          \cellcolor[HTML]{FFF2F2}\textit{-0.34\%} &
          \multicolumn{1}{l|}{\cellcolor[HTML]{FFFEFE}\textit{-0.01\%}} &
          \cellcolor[HTML]{FF5858}\textit{-6.35\%} &
          \cellcolor[HTML]{FF5858}\textit{-9.66\%} &
          \cellcolor[HTML]{FF5858}\textit{-6.49\%} &
          \cellcolor[HTML]{FF5858}\textit{-5.92\%} \\ \midrule
         &
          Traditional &
          \textbf{0.856} &
          0.976 &
          \multicolumn{1}{l|}{\textbf{0.995}} &
          \textbf{0.122} &
          \textbf{0.073} &
          0.426 &
          \textbf{0.155} \\
         &
          Inverted (Ours) &
          \textbf{0.856} &
          \textbf{0.977} &
          \multicolumn{1}{l|}{\textbf{0.995}} &
          \textbf{0.122} &
          \textbf{0.073} &
          \textbf{0.425} &
          \textbf{0.155} \\
        \multirow{-3}{*}{\begin{tabular}[c]{@{}l@{}}AT~\cite{Zagoruyko2019PayingTransfer} \\  \textit{\scriptsize ICLR 2017}\end{tabular}} &
          \textit{Improvement} &
          \cellcolor[HTML]{FFFBFB}\textit{-0.11\%} &
          \cellcolor[HTML]{FDFFFD}\textit{0.06\%} &
          \multicolumn{1}{l|}{\cellcolor[HTML]{FFFFFF}\textit{0.01\%}} &
          \cellcolor[HTML]{FFFCFC}\textit{-0.08\%} &
          \cellcolor[HTML]{E2FFE2}\textit{0.82\%} &
          \cellcolor[HTML]{FFFFFF}\textit{0.02\%} &
          \cellcolor[HTML]{FFFFFF}\textit{0.00\%} \\ \midrule
         &
          Traditional &
          \textbf{0.854} &
          \textbf{0.978} &
          \multicolumn{1}{l|}{\textbf{0.996}} &
          \textbf{0.122} &
          \textbf{0.072} &
          0.429 &
          \textbf{0.155} \\
         &
          Inverted (Ours) &
          \textbf{0.854} &
          0.977 &
          \multicolumn{1}{l|}{\textbf{0.996}} &
          \textbf{0.122} &
          0.073 &
          \textbf{0.427} &
          \textbf{0.155} \\
        \multirow{-3}{*}{\begin{tabular}[c]{@{}l@{}}PKT~\cite{Passalis2018LearningTransfer} \\     \textit{\scriptsize ECCV 2018}\end{tabular}} &
          \textit{Improvement} &
          \cellcolor[HTML]{FEFFFE}\textit{0.04\%} &
          \cellcolor[HTML]{FFFBFB}\textit{-0.09\%} &
          \multicolumn{1}{l|}{\cellcolor[HTML]{FFFFFF}\textit{0.02\%}} &
          \cellcolor[HTML]{FFF9F9}\textit{-0.16\%} &
          \cellcolor[HTML]{FFCCCC}\textit{-1.38\%} &
          \cellcolor[HTML]{F0FFF0}\textit{0.42\%} &
          \cellcolor[HTML]{F8FFF8}\textit{0.19\%} \\ \midrule
         &
          Traditional &
          \textbf{0.861} &
          \textbf{0.978} &
          \multicolumn{1}{l|}{\textbf{0.996}} &
          \textbf{0.119} &
          \textbf{0.070} &
          \textbf{0.416} &
          \textbf{0.151} \\
         &
          Inverted (Ours) &
          0.849 &
          0.975 &
          \multicolumn{1}{l|}{\textbf{0.996}} &
          0.124 &
          0.076 &
          0.433 &
          0.157 \\
        \multirow{-3}{*}{\begin{tabular}[c]{@{}l@{}}Ensemble~\cite{Chen2022ImprovedEnsemble} \\    \textit{\scriptsize NeurIPS 2022}\end{tabular}} &
          \textit{Improvement} &
          \cellcolor[HTML]{FFC9C9}\textit{-1.46\%} &
          \cellcolor[HTML]{FFF4F4}\textit{-0.29\%} &
          \multicolumn{1}{l|}{\cellcolor[HTML]{FFFDFD}\textit{-0.05\%}} &
          \cellcolor[HTML]{FF5656}\textit{-4.64\%} &
          \cellcolor[HTML]{FF5858}\textit{-7.86\%} &
          \cellcolor[HTML]{FF6969}\textit{-4.11\%} &
          \cellcolor[HTML]{FF6464}\textit{-4.25\%} \\ 
          \bottomrule
    \end{tabular}
    \vspace{1em}
    \caption{\textbf{Depth teacher $\rightarrow$ Depth student (no task gap).} As expected, in same-task settings, our inverted projection produces a smaller improvement than the traditional projection. \textit{Improvement} is \% change using our inverted projection over using the traditional projection. See section \ref{sec:app:model_details} for model details. Baseline $\pm$ figures are variance from 3 runs.}
    \label{tab:supp:full-depth-table:depth-teacher}
\end{table}
\begin{table}
    \centering
    \scriptsize
    \begin{tabular}{ll|lllllll}
        \toprule
        \belowrulesepcolor{mygrey}
        \rowcolor{mygrey}
         &
           &
          \multicolumn{7}{c}{{\color{s2d} $\blacksquare$ } \textbf{Instance Segmentation} $\longrightarrow$ Depth} \\
        \rowcolor{mygrey} Method &
          Projection type &
          $\delta_1 \uparrow$ &
          $\delta_2 \uparrow$ &
          \multicolumn{1}{l|}{$\delta_3 \uparrow$} &
          Abs. Rel. $\downarrow$ &
          Sq. Rel. $\downarrow$ &
          RMS $\downarrow$ &
          RMSL $\downarrow$ \\  
        \aboverulesepcolor{mygrey}
        \midrule
        \multicolumn{2}{c|}{\textit{No teacher (baseline)}} &
          \stackengine{2pt}{\textit{0.845}}{$_{\pm 0.007}$}{U}{c}{F}{T}{S} &
          \stackengine{2pt}{\textit{0.974}}{$_{\pm 0.001}$}{U}{c}{F}{T}{S} &
          \multicolumn{1}{l|}{\stackengine{2pt}{\textit{0.995}}{$_{\pm 0.000}$}{U}{c}{F}{T}{S}} &
          \stackengine{2pt}{\textit{0.127}}{$_{\pm 0.003}$}{U}{c}{F}{T}{S} &
          \stackengine{2pt}{\textit{0.078}}{$_{\pm 0.002}$}{U}{c}{F}{T}{S} &
          \stackengine{2pt}{\textit{0.440}}{$_{\pm 0.005}$}{U}{c}{F}{T}{S} &
          \stackengine{2pt}{\textit{0.160}}{$_{\pm 0.003}$}{U}{c}{F}{T}{S} \\
         \midrule
         &
          Traditional &
          \textbf{0.855} &
          \textbf{0.977} &
          \multicolumn{1}{l|}{\textbf{0.996}} &
          \textbf{0.122} &
          \textbf{0.073} &
          \textbf{0.425} &
          \textbf{0.154} \\
         &
          Inverted (Ours) &
          0.851 &
          0.975 &
          \multicolumn{1}{l|}{0.995} &
          0.124 &
          0.075 &
          0.431 &
          0.157 \\
        \multirow{-3}{*}{\begin{tabular}[c]{@{}l@{}}FitNets~\cite{romero_fitnets_2015} \\     \textit{\scriptsize ICLR 2015}\end{tabular}} &
          \textit{Improvement} &
          \cellcolor[HTML]{FFF0F0}\textit{-0.41\%} &
          \cellcolor[HTML]{FFF5F5}\textit{-0.25\%} &
          \multicolumn{1}{l|}{\cellcolor[HTML]{FFFEFE}\textit{-0.02\%}} &
          \cellcolor[HTML]{FFBEBE}\textit{-1.78\%} &
          \cellcolor[HTML]{FFA3A3}\textit{-2.52\%} &
          \cellcolor[HTML]{FFCFCF}\textit{-1.31\%} &
          \cellcolor[HTML]{FFC1C1}\textit{-1.68\%} \\ \midrule
         &
          Traditional &
          0.852 &
          0.976 &
          \multicolumn{1}{l|}{\textbf{0.995}} &
          0.123 &
          0.075 &
          0.431 &
          0.156 \\
         &
          Inverted (Ours) &
          \textbf{0.855} &
          \textbf{0.978} &
          \multicolumn{1}{l|}{\textbf{0.995}} &
          \textbf{0.121} &
          \textbf{0.073} &
          \textbf{0.429} &
          \textbf{0.155} \\
        \multirow{-3}{*}{\begin{tabular}[c]{@{}l@{}}AT~\cite{Zagoruyko2019PayingTransfer} \\  \textit{\scriptsize ICLR 2017}\end{tabular}} &
          \textit{Improvement} &
          \cellcolor[HTML]{F0FFF0}\textit{0.42\%} &
          \cellcolor[HTML]{FAFFFA}\textit{0.16\%} &
          \multicolumn{1}{l|}{\cellcolor[HTML]{FFFFFF}\textit{0.00\%}} &
          \cellcolor[HTML]{CDFFCD}\textit{1.38\%} &
          \cellcolor[HTML]{C0FFC0}\textit{1.74\%} &
          \cellcolor[HTML]{ECFFEC}\textit{0.53\%} &
          \cellcolor[HTML]{E3FFE3}\textit{0.77\%} \\ \midrule
         &
          Traditional &
          \textbf{0.857} &
          \textbf{0.976} &
          \multicolumn{1}{l|}{\textbf{0.995}} &
          \textbf{0.123} &
          \textbf{0.075} &
          \textbf{0.427} &
          \textbf{0.155} \\
         &
          Inverted (Ours) &
          0.854 &
          \textbf{0.976} &
          \multicolumn{1}{l|}{\textbf{0.995}} &
          \textbf{0.123} &
          \textbf{0.075} &
          0.429 &
          0.156 \\
        \multirow{-3}{*}{\begin{tabular}[c]{@{}l@{}}PKT~\cite{Passalis2018LearningTransfer} \\     \textit{\scriptsize ECCV 2018}\end{tabular}} &
          \textit{Improvement} &
          \cellcolor[HTML]{FFF2F2}\textit{-0.34\%} &
          \cellcolor[HTML]{FEFFFE}\textit{0.04\%} &
          \multicolumn{1}{l|}{\cellcolor[HTML]{FFFFFF}\textit{0.01\%}} &
          \cellcolor[HTML]{FFFCFC}\textit{-0.08\%} &
          \cellcolor[HTML]{FFFAFA}\textit{-0.13\%} &
          \cellcolor[HTML]{FFEEEE}\textit{-0.44\%} &
          \cellcolor[HTML]{FFECEC}\textit{-0.52\%} \\ \midrule
         &
          Traditional &
          \textbf{0.856} &
          \textbf{0.977} &
          \multicolumn{1}{l|}{\textbf{0.996}} &
          \textbf{0.122} &
          \textbf{0.072} &
          \textbf{0.425} &
          \textbf{0.154} \\
         &
          Inverted (Ours) &
          0.848 &
          0.975 &
          \multicolumn{1}{l|}{0.995} &
          0.124 &
          0.076 &
          0.435 &
          0.157 \\
        \multirow{-3}{*}{\begin{tabular}[c]{@{}l@{}}Ensemble~\cite{Chen2022ImprovedEnsemble} \\     \textit{\scriptsize NeurIPS 2022}\end{tabular}} &
          \textit{Improvement} &
          \cellcolor[HTML]{FFDCDC}\textit{-0.95\%} &
          \cellcolor[HTML]{FFF9F9}\textit{-0.16\%} &
          \multicolumn{1}{l|}{\cellcolor[HTML]{FFFDFD}\textit{-0.05\%}} &
          \cellcolor[HTML]{FFC3C3}\textit{-1.64\%} &
          \cellcolor[HTML]{FF5353}\textit{-4.70\%} &
          \cellcolor[HTML]{FFB0B0}\textit{-2.16\%} &
          \cellcolor[HTML]{FFBABA}\textit{-1.88\%} \\
          \bottomrule
    \end{tabular}
    \vspace{1em}
    \caption{\textbf{Instance segmentation teacher $\rightarrow$ Depth student (small task gap).} The two tasks are different, but are similar enough that the traditional projection produces greater improvements than our inverted projection does with most methods. \textit{Improvement} is \% change using our inverted projection over using the traditional projection. See section \ref{sec:app:model_details} for model details. Baseline $\pm$ figures are variance from 3 runs.}
    \label{tab:supp:full-depth-table:insseg-teacher}
\end{table}
\begin{table}
    \centering
    \scriptsize
    \begin{tabular}{ll|lllllll}
        \toprule
        \belowrulesepcolor{mygrey}
        \rowcolor{mygrey}
         &
           &
          \multicolumn{7}{c}{{\color{c2d} $\blacksquare$ } \textbf{Classification} $\longrightarrow$ Depth} \\
        \rowcolor{mygrey} Method &
          Projection type &
          $\delta_1 \uparrow$ &
          $\delta_2 \uparrow$ &
          \multicolumn{1}{l|}{$\delta_3 \uparrow$} &
          Abs. Rel. $\downarrow$ &
          Sq. Rel. $\downarrow$ &
          RMS $\downarrow$ &
          RMSL $\downarrow$ \\ 
        \aboverulesepcolor{mygrey}
        \midrule
        \multicolumn{2}{c|}{\textit{No teacher (baseline)}} &
          \stackengine{2pt}{\textit{0.845}}{$_{\pm 0.007}$}{U}{c}{F}{T}{S} &
          \stackengine{2pt}{\textit{0.974}}{$_{\pm 0.001}$}{U}{c}{F}{T}{S} &
          \multicolumn{1}{l|}{\stackengine{2pt}{\textit{0.995}}{$_{\pm 0.000}$}{U}{c}{F}{T}{S}} &
          \stackengine{2pt}{\textit{0.127}}{$_{\pm 0.003}$}{U}{c}{F}{T}{S} &
          \stackengine{2pt}{\textit{0.078}}{$_{\pm 0.002}$}{U}{c}{F}{T}{S} &
          \stackengine{2pt}{\textit{0.440}}{$_{\pm 0.005}$}{U}{c}{F}{T}{S} &
          \stackengine{2pt}{\textit{0.160}}{$_{\pm 0.003}$}{U}{c}{F}{T}{S} \\
         \midrule
         &
          Traditional &
          0.845 &
          \textbf{0.976} &
          \multicolumn{1}{l|}{\textbf{0.996}} &
          0.125 &
          0.076 &
          0.439 &
          0.158 \\
         &
          Inverted (Ours) &
          \textbf{0.850} &
          0.975 &
          \multicolumn{1}{l|}{\textbf{0.995}} &
          \textbf{0.124} &
          \textbf{0.075} &
          \textbf{0.434} &
          \textbf{0.157} \\
        \multirow{-3}{*}{\begin{tabular}[c]{@{}l@{}}FitNets~\cite{romero_fitnets_2015} \\     \textit{\scriptsize ICLR 2015}\end{tabular}} &
          \textit{Improvement} &
          \cellcolor[HTML]{EDFFED}\textit{0.50\%} &
          \cellcolor[HTML]{FFFCFC}\textit{-0.06\%} &
          \multicolumn{1}{l|}{\cellcolor[HTML]{FFFDFD}\textit{-0.03\%}} &
          \cellcolor[HTML]{ECFFEC}\textit{0.53\%} &
          \cellcolor[HTML]{EFFFEF}\textit{0.44\%} &
          \cellcolor[HTML]{CFFFCF}\textit{1.34\%} &
          \cellcolor[HTML]{E2FFE2}\textit{0.80\%} \\ \midrule
         &
          Traditional &
          0.850 &
          \textbf{0.976} &
          \multicolumn{1}{l|}{\textbf{0.995}} &
          0.125 &
          0.076 &
          0.433 &
          0.157 \\
         &
          Inverted (Ours) &
          \textbf{0.853} &
          \textbf{0.976} &
          \multicolumn{1}{l|}{\textbf{0.995}} &
          \textbf{0.123} &
          \textbf{0.074} &
          \textbf{0.430} &
          \textbf{0.156} \\
        \multirow{-3}{*}{\begin{tabular}[c]{@{}l@{}}AT~\cite{Zagoruyko2019PayingTransfer} \\ \textit{\scriptsize ICLR 2017}\end{tabular}} &
          \textit{Improvement} &
          \cellcolor[HTML]{F3FFF3}\textit{0.35\%} &
          \cellcolor[HTML]{FDFFFD}\textit{0.08\%} &
          \multicolumn{1}{l|}{\cellcolor[HTML]{FFFFFF}\textit{0.02\%}} &
          \cellcolor[HTML]{C5FFC5}\textit{1.61\%} &
          \cellcolor[HTML]{91FF91}\textit{3.03\%} &
          \cellcolor[HTML]{E3FFE3}\textit{0.79\%} &
          \cellcolor[HTML]{E1FFE1}\textit{0.83\%} \\ \midrule
         &
          Traditional &
          0.851 &
          0.975 &
          \multicolumn{1}{l|}{\textbf{0.996}} &
          0.124 &
          0.076 &
          0.432 &
          0.157 \\
         &
          Inverted (Ours) &
          \textbf{0.853} &
          \textbf{0.976} &
          \multicolumn{1}{l|}{0.995} &
          \textbf{0.123} &
          \textbf{0.074} &
          \textbf{0.431} &
          \textbf{0.156} \\
        \multirow{-3}{*}{\begin{tabular}[c]{@{}l@{}}PKT~\cite{Passalis2018LearningTransfer} \\     \textit{\scriptsize ECCV 2018}\end{tabular}} &
          \textit{Improvement} &
          \cellcolor[HTML]{F7FFF7}\textit{0.25\%} &
          \cellcolor[HTML]{FEFFFE}\textit{0.05\%} &
          \multicolumn{1}{l|}{\cellcolor[HTML]{FFFDFD}\textit{-0.03\%}} &
          \cellcolor[HTML]{D1FFD1}\textit{1.29\%} &
          \cellcolor[HTML]{A5FFA5}\textit{2.50\%} &
          \cellcolor[HTML]{F5FFF5}\textit{0.30\%} &
          \cellcolor[HTML]{E8FFE8}\textit{0.64\%} \\ \midrule
         &
          Traditional &
          \textbf{0.852} &
          \textbf{0.976} &
          \multicolumn{1}{l|}{\textbf{0.995}} &
          \textbf{0.124} &
          \textbf{0.075} &
          \textbf{0.431} &
          \textbf{0.156} \\
         &
          Inverted (Ours) &
          0.847 &
          0.975 &
          \multicolumn{1}{l|}{\textbf{0.995}} &
          0.125 &
          0.076 &
          0.437 &
          0.158 \\
        \multirow{-3}{*}{\begin{tabular}[c]{@{}l@{}}Ensemble~\cite{Chen2022ImprovedEnsemble} \\     \textit{\scriptsize NeurIPS 2022}\end{tabular}} &
          \textit{Improvement} &
          \cellcolor[HTML]{FFE7E7}\textit{-0.63\%} &
          \cellcolor[HTML]{FFFAFA}\textit{-0.12\%} &
          \multicolumn{1}{l|}{\cellcolor[HTML]{FFFFFF}\textit{0.02\%}} &
          \cellcolor[HTML]{FFDEDE}\textit{-0.89\%} &
          \cellcolor[HTML]{FFC4C4}\textit{-1.61\%} &
          \cellcolor[HTML]{FFCFCF}\textit{-1.30\%} &
          \cellcolor[HTML]{FFD7D7}\textit{-1.09\%} \\
          \bottomrule
    \end{tabular}
    \vspace{1em}
    \caption{\textbf{Classification teacher $\rightarrow$ Depth student (larger task gap).} The two tasks are different enough that the setting becomes more ``cross-task" than ``same-task", and our inverted projection begins to outperform the traditional student model in terms of improvement over the baseline. \textit{Improvement} is \% change using our inverted projection over using the traditional projection. See section \ref{sec:app:model_details} for model details. Baseline $\pm$ figures are variance from 3 runs.}
    \label{tab:supp:full-depth-table:class-teacher}
\end{table}
\begin{table}
    \centering
    \scriptsize
    \begin{tabular}{ll|lllllll}
        \toprule
        \belowrulesepcolor{mygrey}
        \rowcolor{mygrey}
         &
           &
          \multicolumn{7}{c}{{\color{r2d} $\blacksquare$ } \textbf{Random \textit{(Least similar)}} $\longrightarrow$ Depth} \\
        \rowcolor{mygrey} Method &
          Projection type &
          $\delta_1 \uparrow$ &
          $\delta_2 \uparrow$ &
          \multicolumn{1}{l|}{$\delta_3 \uparrow$} &
          Abs. Rel. $\downarrow$ &
          Sq. Rel. $\downarrow$ &
          RMS $\downarrow$ &
          RMSL $\downarrow$ \\ 
        \aboverulesepcolor{mygrey}
        \midrule
        \multicolumn{2}{c|}{\textit{No teacher (baseline)}} &
          \stackengine{2pt}{\textit{0.845}}{$_{\pm 0.007}$}{U}{c}{F}{T}{S} &
          \stackengine{2pt}{\textit{0.974}}{$_{\pm 0.001}$}{U}{c}{F}{T}{S} &
          \multicolumn{1}{l|}{\stackengine{2pt}{\textit{0.995}}{$_{\pm 0.000}$}{U}{c}{F}{T}{S}} &
          \stackengine{2pt}{\textit{0.127}}{$_{\pm 0.003}$}{U}{c}{F}{T}{S} &
          \stackengine{2pt}{\textit{0.078}}{$_{\pm 0.002}$}{U}{c}{F}{T}{S} &
          \stackengine{2pt}{\textit{0.440}}{$_{\pm 0.005}$}{U}{c}{F}{T}{S} &
          \stackengine{2pt}{\textit{0.160}}{$_{\pm 0.003}$}{U}{c}{F}{T}{S} \\
         \midrule
         &
          Traditional &
          0.828 &
          0.970 &
          \multicolumn{1}{l|}{\textbf{0.995}} &
          0.134 &
          0.084 &
          0.455 &
          0.167 \\
         &
          Inverted (Ours) &
          \textbf{0.851} &
          \textbf{0.976} &
          \multicolumn{1}{l|}{\textbf{0.995}} &
          \textbf{0.124} &
          \textbf{0.075} &
          \textbf{0.431} &
          \textbf{0.156} \\
        \multirow{-3}{*}{\begin{tabular}[c]{@{}l@{}}FitNets~\cite{romero_fitnets_2015} \\     \textit{\scriptsize ICLR 2015}\end{tabular}} &
          \textit{Improvement} &
          \cellcolor[HTML]{97FF97}\textit{2.86\%} &
          \cellcolor[HTML]{EAFFEA}\textit{0.58\%} &
          \multicolumn{1}{l|}{\cellcolor[HTML]{FDFFFD}\textit{0.08\%}} &
          \cellcolor[HTML]{00FF00}\textit{7.47\%} &
          \cellcolor[HTML]{00FF00}\textit{11.15\%} &
          \cellcolor[HTML]{42FF42}\textit{5.20\%} &
          \cellcolor[HTML]{18FF18}\textit{6.36\%} \\ \midrule
         &
          Traditional &
          \textbf{0.857} &
          \textbf{0.977} &
          \multicolumn{1}{l|}{\textbf{0.996}} &
          \textbf{0.121} &
          \textbf{0.073} &
          \textbf{0.428} &
          \textbf{0.154} \\
         &
          Inverted (Ours) &
          \textbf{0.857} &
          0.976 &
          \multicolumn{1}{l|}{0.995} &
          0.122 &
          0.074 &
          \textbf{0.428} &
          0.155 \\
        \multirow{-3}{*}{\begin{tabular}[c]{@{}l@{}}AT~\cite{Zagoruyko2019PayingTransfer} \\ \textit{\scriptsize ICLR 2017}\end{tabular}} &
          \textit{Improvement} &
          \cellcolor[HTML]{FEFFFE}\textit{0.05\%} &
          \cellcolor[HTML]{FFFDFD}\textit{-0.04\%} &
          \multicolumn{1}{l|}{\cellcolor[HTML]{FFFDFD}\textit{-0.03\%}} &
          \cellcolor[HTML]{FFE0E0}\textit{-0.83\%} &
          \cellcolor[HTML]{FFCCCC}\textit{-1.37\%} &
          \cellcolor[HTML]{FCFFFC}\textit{0.09\%} &
          \cellcolor[HTML]{FFF0F0}\textit{-0.39\%} \\ \midrule
         &
          Traditional &
          0.856 &
          0.975 &
          \multicolumn{1}{l|}{\textbf{0.995}} &
          0.123 &
          0.075 &
          0.429 &
          \textbf{0.155} \\
         &
          Inverted (Ours) &
          \textbf{0.858} &
          \textbf{0.976} &
          \multicolumn{1}{l|}{\textbf{0.995}} &
          \textbf{0.122} &
          \textbf{0.073} &
          \textbf{0.426} &
          \textbf{0.155} \\
        \multirow{-3}{*}{\begin{tabular}[c]{@{}l@{}}PKT~\cite{Passalis2018LearningTransfer} \\     \textit{\scriptsize ECCV 2018}\end{tabular}} &
          \textit{Improvement} &
          \cellcolor[HTML]{F5FFF5}\textit{0.29\%} &
          \cellcolor[HTML]{FCFFFC}\textit{0.10\%} &
          \multicolumn{1}{l|}{\cellcolor[HTML]{FFFFFF}\textit{0.00\%}} &
          \cellcolor[HTML]{D3FFD3}\textit{1.22\%} &
          \cellcolor[HTML]{99FF99}\textit{2.80\%} &
          \cellcolor[HTML]{E1FFE1}\textit{0.84\%} &
          \cellcolor[HTML]{EAFFEA}\textit{0.58\%} \\ \midrule
         &
          Traditional &
          0.835 &
          0.973 &
          \multicolumn{1}{l|}{0.995} &
          0.128 &
          0.079 &
          0.446 &
          0.162 \\
         &
          Inverted (Ours) &
          \textbf{0.849} &
          \textbf{0.976} &
          \multicolumn{1}{l|}{\textbf{0.996}} &
          \textbf{0.124} &
          \textbf{0.075} &
          \textbf{0.432} &
          \textbf{0.157} \\
        \multirow{-3}{*}{\begin{tabular}[c]{@{}l@{}}Ensemble~\cite{Chen2022ImprovedEnsemble} \\     \textit{\scriptsize NeurIPS 2022}\end{tabular}} &
          \textit{Improvement} &
          \cellcolor[HTML]{C0FFC0}\textit{1.74\%} &
          \cellcolor[HTML]{F6FFF6}\textit{0.26\%} &
          \multicolumn{1}{l|}{\cellcolor[HTML]{FDFFFD}\textit{0.06\%}} &
          \cellcolor[HTML]{9BFF9B}\textit{2.75\%} &
          \cellcolor[HTML]{4BFF4B}\textit{4.96\%} &
          \cellcolor[HTML]{91FF91}\textit{3.03\%} &
          \cellcolor[HTML]{84FF84}\textit{3.39\%} \\
        \bottomrule
    \end{tabular}
    \vspace{1em}
    \caption{\textbf{Randomly-initialised teacher $\rightarrow$ Depth student (largest task gap).} Our inverted projection produces significant improvement. \textit{Improvement} is \% change using our inverted projection over using the traditional projection. See section \ref{sec:app:model_details} for model details. Baseline $\pm$ figures are variance from 3 runs.}
    \label{tab:supp:full-depth-table:random-teacher}
\end{table}
